# Supplementary material for: Chaos and Synchronization in Financial Leverages Dynamics: Modeling Systemic Risk with Coupled Unimodal Maps
Source: arXiv:2601.01505 ancillary file (2026-03-30)
Supplement: Supplementary file 1 [file Supplementary_material.pdf]

# Supplementary Material

December 24, 2025

This document contains the proof of the theorems mentioned in the paper, together with some more details concerning the model and the numerical simulations performed.

## Contents

|          |                                                                              |          |
|----------|------------------------------------------------------------------------------|----------|
| <b>1</b> | <b>Model for One Bank</b>                                                    | <b>1</b> |
| 1.1      | Constraints on the Initial Conditions for the Leverage and on $\omega$ . . . | 2        |
| <b>2</b> | <b>Model with Two Banks</b>                                                  | <b>2</b> |
| 2.1      | Constraints . . . . .                                                        | 2        |
| 2.2      | Homogeneous Case . . . . .                                                   | 3        |
| 2.2.1    | Numerical Observations . . . . .                                             | 3        |
| 2.2.2    | Analytical Considerations . . . . .                                          | 5        |
| 2.3      | Heterogeneous Case . . . . .                                                 | 6        |
| 2.3.1    | Numerical Observations . . . . .                                             | 6        |
| 2.3.2    | Analytical Considerations in the Skew-Product Case . . . . .                 | 7        |
| 2.3.3    | The general $\pi \neq 0, 1$ case . . . . .                                   | 30       |

## 1 Model for One Bank

Recall the map  $T$ :

$$\lambda_{t+1} = T(\lambda_t) = \left( \frac{\omega}{\lambda_t^2} + \frac{(1-\omega)\gamma^2\alpha^2\Sigma_\epsilon}{(1+\gamma-\lambda_t)^2} \right)^{-2}$$

## 1.1 Constraints on the Initial Conditions for the Leverage and on $\omega$

As mentioned, to be economically relevant, the leverage has natural limits  $\lambda_t \geq 1$  being the ratio of positive numbers where the numerator is larger than the denominator, and  $\lambda_t \leq 1 + \gamma$  to ensure stationarity of the AR(1) process describing the return of the asset requires. One can ensure that these constraints are satisfied by choosing initial conditions in a subinterval of  $[0, 1 + \gamma]$  and restricting the admissible choices of  $\omega$  (having fixed all the other parameters as specified in the paper). Let's make the dependence of the unimodal map  $T$  on  $\omega$  explicit by referring to it as  $T_\omega$ . For the choice made of the other parameters, the maximum of  $T_\omega$  in  $[0, 1 + \gamma]$  is greater than 1 and less than  $1 + \gamma$ . Call  $c_\omega$  the critical point of  $T_\omega$  and put  $T_\omega^{-1}(\{1\}) = \{\lambda_{\min}(\omega), \lambda_{\max}(\omega)\} \subseteq [0, 1 + \gamma]$  such that  $\lambda_{\min}(\omega) \leq c_\omega \leq \lambda_{\max}(\omega)$ . It can be numerically verified that it holds:  $\forall \omega \in [0.3, 0.9], \lambda_{\min}(\omega) < 1, \min(T_\omega(1), T_\omega(\lambda_{\max}(\omega))) > 1$  and  $T_\omega(c_\omega) < \lambda_{\max}(\omega)$ . Moreover,  $\inf_{\omega \in [0.3, 0.9]} \lambda_{\max}(\omega) > \sup_{\omega \in [0.3, 0.9]} c_\omega$ . This allows, by taking initial conditions  $\lambda_0$  in the invariant interval  $[1, \inf_{\omega \in [0.3, 0.9]} \lambda_{\max}(\omega)]$ , to have the constraints on  $\lambda$  always verified.

## 2 Model with Two Banks

Recall the maps  $T_1, T_2$ :

$$\lambda_{1,t+1} = T_1(\lambda_{1,t}, \lambda_{2,t}) = \left( \frac{\omega_1}{\lambda_{1,t}^2} + \frac{(1 - \omega_1)\gamma^2\alpha^2\Sigma_\epsilon}{(1 + \gamma - \pi_1\lambda_{1,t} - (1 - \pi_1)\lambda_{2,t})^2} \right)^{-2}$$

$$\lambda_{2,t+1} = T_2(\lambda_{1,t}, \lambda_{2,t}) = \left( \frac{\omega_2}{\lambda_{2,t}^2} + \frac{(1 - \omega_2)\gamma^2\alpha^2\Sigma_\epsilon}{(1 + \gamma - \pi_1\lambda_{1,t} - (1 - \pi_1)\lambda_{2,t})^2} \right)^{-2}$$

### 2.1 Constraints

Let us show that, at least for  $|\omega_1 - \omega_2|$  small enough and such that  $(\omega_1, \omega_2) \in [0.3, 0.9]^2$ , the set  $\mathcal{V}$  introduced in the paper is non-empty.

Put  $s_t = \lambda_{1,t} + \lambda_{2,t}$ ,  $\delta_t = \lambda_{1,t} - \lambda_{2,t}$ . Notice that, for  $\omega_1 = \omega_2 \doteq \omega$  and  $\delta_t = 0$ ,  $s_{t+1} \doteq D_\omega(s_t) = \left( \frac{\omega}{(s_t)^2} + \frac{(1-\omega)A}{(2B-s_t)^2} \right)^{-\frac{1}{2}}$ .  $D_\omega$  is a unimodal map on  $[0, 2B]$ .

For the given choice of the parameters, the maximum of  $D_\omega$  in  $[0, 2B]$  is greater than 1 and less than  $2B$ . Call  $c_\omega$  the critical point of  $D_\omega$  and put  $D_\omega^{-1}(\{1\}) = \{\lambda_{\min}(\omega), \lambda_{\max}(\omega)\} \subseteq [0, 2(1 + \gamma)]$  such that  $\lambda_{\min}(\omega) \leq c_\omega \leq \lambda_{\max}(\omega)$ .

It holds:  $\forall \omega \in [0.3, 0.9], \lambda_{\min}(\omega) < 2, D_\omega(2) > 2$  and  $D_\omega(c_\omega) < \lambda_{\max}(\omega)$ .

Moreover,  $\inf_{\omega \in [0.3, 0.9]} \lambda_{\max}(\omega) > \sup_{\omega \in [0.3, 0.9]} c_{\omega}$ . This allows one to consider initial conditions  $s_0$  in the invariant interval  $[2, \inf_{\omega \in [0.3, 0.9]} \lambda_{\max}(\omega)]$ , and one has  $\text{dist}(D_{\omega}([2, \inf_{\omega \in [0.3, 0.9]} \lambda_{\max}(\omega)]), [2, \inf_{\omega \in [0.3, 0.9]} \lambda_{\max}(\omega)]) > 0 \forall \omega \in [0.3, 0.9]$ .

By continuity, there will exist intervals  $[s_{\min}, s_{\max}]$  and  $[s_{\min,2}, s_{\max,2}]$  with  $[0, 2B] \supseteq [s_{\min}, s_{\max}] \supseteq [s_{\min,2}, s_{\max,2}]$ ,  $\text{dist}([s_{\min}, s_{\max}], [s_{\min,2}, s_{\max,2}]) > 0$  and  $\epsilon_r > 0$  such that  $\forall t \in \mathbb{N}, \forall \omega \in [0.3, 0.9], \forall (s_t, \frac{\delta_t}{s_t}) \in [s_{\min}, s_{\max}] \times [-\epsilon_r, \epsilon_r], s_{t+1} \in [s_{\min,2}, s_{\max,2}]$ . As will be shown in the proof of Theorem 1, one also has that if  $\omega_1 = \omega_2$  then for each  $\delta_t$  and  $s_t$  such that the constraints are satisfied at time  $t$ , one has  $\frac{|\delta_{t+1}|}{s_{t+1}} \leq \frac{1}{1+K} \frac{|\delta_t|}{s_t}$  with  $\mathbb{R} \ni K > 0$ . Thus by choosing initial conditions such that  $(s_0, \frac{\delta_0}{s_0}) \in [s_{\min}, s_{\max}] \times [-\epsilon_r, \epsilon_r]$  one can only focus on the dynamics on the invariant set  $[s_{\min}, s_{\max}] \times [-\epsilon_r, \epsilon_r]$  with, moreover,  $\text{dist}([s_{\min}, s_{\max}] \times [-\epsilon_r, \epsilon_r], (s_{t+1}, r_{t+1})) > 0 \forall (s_t, r_t) \in [s_{\min}, s_{\max}] \times [-\epsilon_r, \epsilon_r]$  for the variables  $(s_t, r_t)$  with  $r_t \doteq \frac{\delta_t}{s_t}$  well defined at every time.

Now notice that the constraints on  $\lambda_{1,t}$  and  $\lambda_{2,t}$ , namely  $\forall t \in \mathbb{N} \lambda_{1,t} \geq 1, \lambda_{2,t} \geq 1, \lambda_{1,t}\pi_1 + \lambda_{2,t}(1 - \pi_1) \leq 1 + \gamma$  can be recasted in the new variables as  $\forall t \in \mathbb{N} s_t \geq 2, r_t s_t (2\pi_1 - 1) + s_t \leq 2(1 + \gamma)$ . This shows that, by choosing initial conditions in  $[s_{\min}, s_{\max}] \times [-\min(\epsilon_r, \frac{2(1+\gamma)-s_{\max}}{s_{\max}}), \min(\epsilon_r, \frac{2(1+\gamma)-s_{\max}}{s_{\max}})]$  the constraints will be satisfied at any time. So far, the case  $\omega_1 = \omega_2$  has been considered.

It is possible to show that  $\mathcal{V}$  is not empty in the case  $\omega_1 \neq \omega_2$  as well, at least if  $|\omega_1 - \omega_2|$  is sufficiently small. Indeed, if  $\omega_1 = \omega_2$ , from previous observations one has  $\text{dist}([s_{\min}, s_{\max}] \times [-\min(\epsilon_r, \frac{2(1+\gamma)-s_{\max}}{s_{\max}}), \min(\epsilon_r, \frac{2(1+\gamma)-s_{\max}}{s_{\max}})], (s_{t+1}, r_{t+1})) > 0 \forall (s_t, r_t) \in [s_{\min}, s_{\max}] \times [-\epsilon_r, \epsilon_r]$ . As a result, if  $\omega_1 \neq \omega_2$  but  $|\omega_1 - \omega_2|$  is sufficiently small, by continuity one can still choose initial conditions in  $[s_{\min}, s_{\max}] \times [-\min(\epsilon_r, \frac{2(1+\gamma)-s_{\max}}{s_{\max}}), \min(\epsilon_r, \frac{2(1+\gamma)-s_{\max}}{s_{\max}})]$  and have the constraints satisfied at any time.

## 2.2 Homogeneous Case

Let's begin by considering the simpler case in which there are  $N$  banks with all the parameter  $\omega_i$  equal.

### 2.2.1 Numerical Observations

For  $N = 2$ , the numerical simulations clearly show that for every choice of  $\pi_1 \in [0, 1]$  the two leverages become, after few iterations, totally synchronized. The nature of the common asymptotic behavior (i.e. periodic of a specific period or aperiodic) depends on the value of  $\omega = \omega_1 = \omega_2$ . In Fig. 1 are shown the orbits of the two leverages for three different choices of  $\omega$ . In these examples  $\pi_1 = 0.5$ .

Fig. 2 displays the two Lyapunov exponents of the deterministic map  $(T_1, T_2)$  as a function of  $\omega$ . The smaller Lyapunov exponent has been calculated using the algorithm which employs the Gram-Schmidt orthogonalization procedure at every

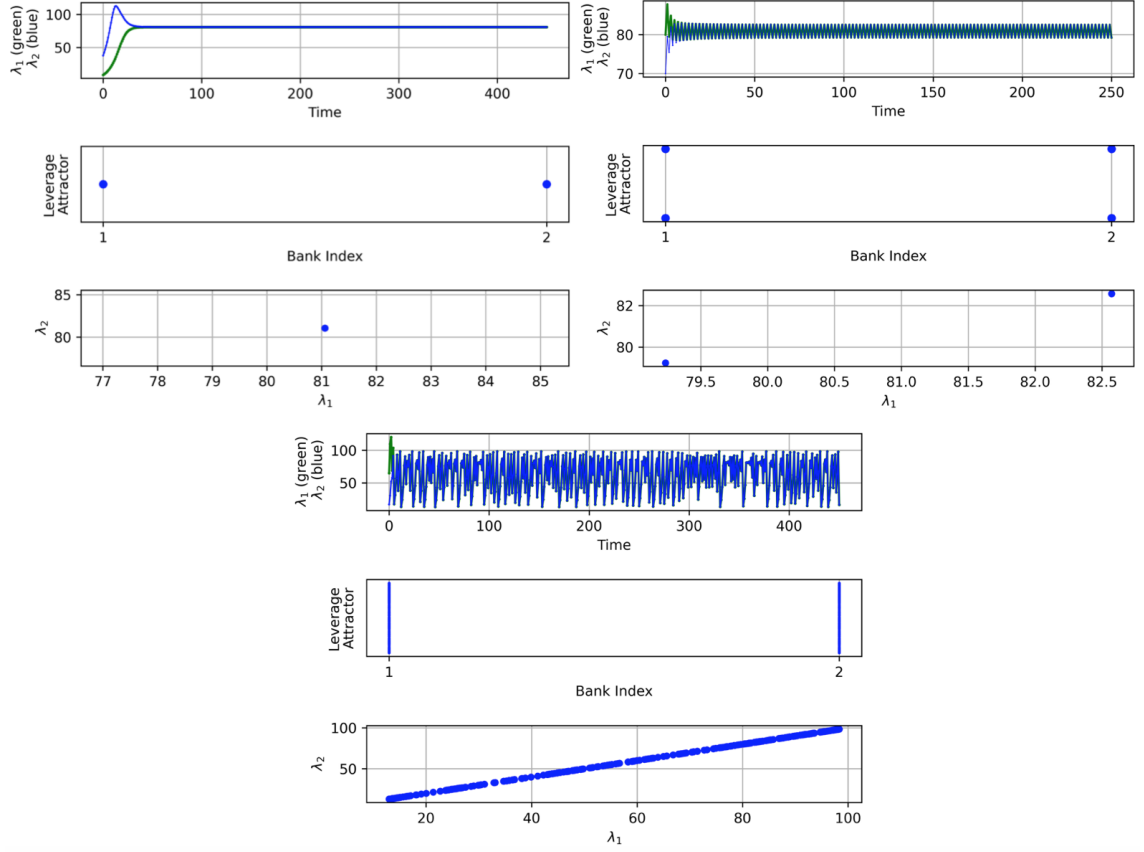

Figure 1: The times series (top panel), the asymptotic orbit for each bank (middle panel) and the plot of the asymptotic orbit on the  $\lambda_1$  vs  $\lambda_2$  plane (bottom panel) are depicted for  $\omega_1 = \omega_2 = 0.8, 0.6, 0.3$  (from top to bottom, left to right). For completeness,  $\pi_1 = \pi_2 = 0.5$ . Regarding the middle and bottom panels of the plots, the first 500 values have been discarded, and the next 1000 have been plotted.

time step. The fact that at least one Lyapunov exponent is always negative and that the maximal one is negative iff the Lyapunov exponent for the corresponding isolated bank is negative is coherent with the observed complete synchronization between the two banks and with the fact that the behavior of the system is the same as the one of the map  $T$  with memory  $\omega$ .

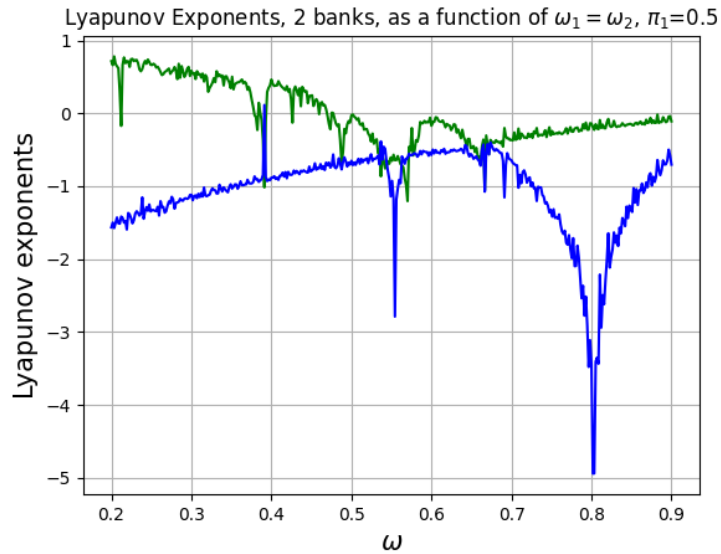

Figure 2: Lyapunov exponents for the bidimensional map  $(T_1, T_2)$ , calculated over 100 time steps.

Trying different choices for the parameters  $(\Sigma_\epsilon, \gamma, \alpha)$  one observes again complete synchronization, for every  $\omega$ , of the two leverages with the same asymptotic behavior as the one found in the corresponding isolated bank system.

### 2.2.2 Analytical Considerations

In the case  $N = 2$ , the numerical simulations showed asymptotic synchronization between banks in the homogeneous case. We are going to prove this analytically for a general number of banks  $N$ . First of all, let's notice that since in the homogeneous case the equations for the leverages have full permutation symmetry, the synchronisation manifold  $\{\lambda_1 = \lambda_2 = \dots = \lambda_N\}$  is invariant. The theorem below proves the asymptotic stability of this manifold, i.e. the leverages of different banks approach asymptotically the same orbit.

**Theorem 1.** (*Synchronization in the Homogeneous Case*) For  $N \geq 2$  coupled banks with the same risk estimation strategy, i.e.  $\omega_1 = \omega_2 = \dots = \omega_N =: \omega$ , for all

admissible initial conditions  $(\lambda_{1,0}, \lambda_{2,0}, \dots, \lambda_{N,0}) \in \mathcal{V}$  one has

$$\lim_{t \rightarrow \infty} |\lambda_{i,t} - \lambda_{j,t}| = 0 \quad \forall i, j \in \{1, \dots, N\}.$$

*Proof.* We will show that for all  $i, j \in \{1, \dots, N\}$  and  $t \in \mathbb{N}$  there is  $K \geq 0$  such that  $\frac{|\lambda_{i,t+1} - \lambda_{j,t+1}|}{\lambda_{i,t+1} + \lambda_{j,t+1}} \leq \frac{1}{1+K} \frac{|\lambda_{i,t} - \lambda_{j,t}|}{\lambda_{i,t} + \lambda_{j,t}}$ , with  $K = 0$  iff  $\lambda_{i,t} = \lambda_{j,t}$ . This implies the proof.

Define  $C = C(\{\lambda_{i,t}\}_{i=1}^N, \omega) = \frac{(1-\omega)A}{(B - \sum_{i=1}^N \pi_i \lambda_{i,t})^2}$ . Without loss of generality we can pick  $i = 1$  and  $j = 2$ . It is not hard to show from the evolution equations that if  $\lambda_{1,t} - \lambda_{2,t} \geq 0$ , then  $\lambda_{1,t+1} - \lambda_{2,t+1} \geq 0$ ; without loss of generality, let us assume this is the case. One has

$$\begin{aligned} \frac{\lambda_{1,t+1} - \lambda_{2,t+1}}{\lambda_{1,t+1} + \lambda_{2,t+1}} &= \frac{\left(\frac{\omega}{\lambda_{1,t}^2} + C\right)^{-\frac{1}{2}} - \left(\frac{\omega}{\lambda_{2,t}^2} + C\right)^{-\frac{1}{2}}}{\left(\frac{\omega}{\lambda_{1,t}^2} + C\right)^{-\frac{1}{2}} + \left(\frac{\omega}{\lambda_{2,t}^2} + C\right)^{-\frac{1}{2}}} = \frac{\left(\frac{\omega}{\lambda_{1,t}^2} + C\right) - \left(\frac{\omega}{\lambda_{2,t}^2} + C\right)}{\left(\left(\frac{\omega}{\lambda_{2,t}^2} + C\right)^{\frac{1}{2}} + \left(\frac{\omega}{\lambda_{1,t}^2} + C\right)^{\frac{1}{2}}\right)^2} \\ &\leq \frac{\lambda_{1,t}^2 - \lambda_{2,t}^2}{\lambda_{1,t}^2 + \lambda_{2,t}^2 + 2 \frac{\lambda_{1,t}^2 \lambda_{2,t}^2}{\omega} \left(\frac{\omega}{\lambda_{1,t}^2} + C\right)^{\frac{1}{2}} \left(\frac{\omega}{\lambda_{2,t}^2} + C\right)^{\frac{1}{2}}} \\ &= \frac{\lambda_{1,t}^2 - \lambda_{2,t}^2}{(\lambda_{1,t} + \lambda_{2,t})^2 \left(1 + \frac{-2\lambda_{1,t}\lambda_{2,t} + 2 \frac{\lambda_{1,t}^2 \lambda_{2,t}^2}{\omega} \left(\frac{\omega}{\lambda_{1,t}^2} + C\right)^{\frac{1}{2}} \left(\frac{\omega}{\lambda_{2,t}^2} + C\right)^{\frac{1}{2}}}{(\lambda_{1,t} + \lambda_{2,t})^2}\right)} \end{aligned}$$

With the equality holding iff  $\lambda_{1,t} = \lambda_{2,t}$

To conclude, note that  $-2\lambda_{1,t}\lambda_{2,t} + 2 \frac{\lambda_{1,t}^2 \lambda_{2,t}^2}{\omega} \left(\frac{\omega}{\lambda_{1,t}^2} + C\right)^{\frac{1}{2}} \left(\frac{\omega}{\lambda_{2,t}^2} + C\right)^{\frac{1}{2}} = -2\lambda_{1,t}\lambda_{2,t} + 2\lambda_{1,t}\lambda_{2,t} \left(1 + \frac{\lambda_{1,t}^2 C}{\omega}\right)^{\frac{1}{2}} \left(1 + \frac{\lambda_{2,t}^2 C}{\omega}\right)^{\frac{1}{2}} \geq 0$   $\square$

*Remark.* Note that the above proof is completely analytic.

## 2.3 Heterogeneous Case

### 2.3.1 Numerical Observations

Already in the case  $N = 2$ , one can see that when  $\omega_1 \neq \omega_2$ , one can see that the two leverages don't synchronize anymore in the long run, and their behavior depends on  $\pi_1$ . Set again  $\gamma = 100, \alpha = 1.64, \Sigma_\epsilon = 0.0015^2$ . Depending on the choice of  $\omega_1, \omega_2$  and  $\pi_1$ , what one observes is that the two leverages either:

1. Both reach a common fixed point.
2. Both asymptotically reach a periodic attractor, which is not the same among the two.

3. Both asymptotically behave in a nonperiodic manner. Further, the two banks are not synchronized and in particular the functional dependence between asymptotic  $\lambda_{1,t}$  and  $\lambda_{2,t}$  seems to get lost as  $|\omega_1 - \omega_2|$  increases.

Figs. 6, 7, and 8 show some examples of the time series and the asymptotic orbits of the two leverages for different choices of  $\omega_1, \omega_2$ . To investigate this system further, one can plot the two asymptotic orbits (for the two leverages) as a function of  $\pi_1 \in [0, 1]$  for several choices of  $\omega_1, \omega_2$ . Some plots, for several choices of  $\omega_1, \omega_2$  are reported in Figs. 3, 4, 5.

What one finds is that for  $\pi_1 = 0$  the asymptotic behavior of bank 2 is the one expected by looking at the bifurcation diagram for the isolated bank system, as it is easily understood.

The behavior for bank 1 will then be of the same qualitative type (i.e. periodic of a given period or aperiodic) as the one of the second bank, although the two leverages won't synchronize.

For  $\pi_1 = 1$  one obtains analogous results as in the  $\pi_1 = 0$  case by only exchanging bank 1 with bank 2.

For  $0 < \pi_1 < 1$  both banks will asymptotically behave in a way of which is "intermediate" (thinking about a period-doubling cascade) between the one reached for  $\pi_1 = 0$  and the one reached for  $\pi_1 = 1$ .

Next, let's consider the case in which we fix  $\pi_1$  and consider the behavior of the leverages as  $\omega_1, \omega_2$  vary. One gets the three dimensional bifurcation diagrams as in Fig. 9 (for three different choices of  $\pi_1$ ). One observes that, broadly speaking, for a given  $\pi_1$  the larger the two memories the more stable the system is. More specifically, for  $\omega_2$  large enough there is a critical value (depending on  $\omega_2$ )  $\omega_1^c(\omega_2)$  such that if  $\omega_1 > \omega_1^c(\omega_2)$  the system reaches a stable fixed point, while it becomes unstable for  $\omega_1 < \omega_1^c(\omega_2)$ . Actually, this critical value depends on  $\pi_1$  too. In particular, the larger  $\pi_1$  the closer the function  $\omega_2 \mapsto \omega_1^c(\omega_2)$  seems to be to a constant function. This is to be expected as for large  $\pi_1$  the smaller bank's memory has a little impact on the whole system. Lastly, one could consider sections of the three dimensional bifurcation diagrams introduced above for fixed values of  $\omega_2$  (for example), as in Fig. 10, where  $\pi_1 = 0.5$ . Notice that again the transition towards a chaotic behavior happens through a cascade of period doubling bifurcations.

### 2.3.2 Analytical Considerations in the Skew-Product Case

Let's consider the case in which  $\pi_1 = 0$  (the  $\pi_1 = 1$  case is analogous). Under these conditions, this may be looked at as a forcing-forced system, in which a larger bank "drives" the behaviour of another bank that is so small not to influence the behaviour of the larger one.

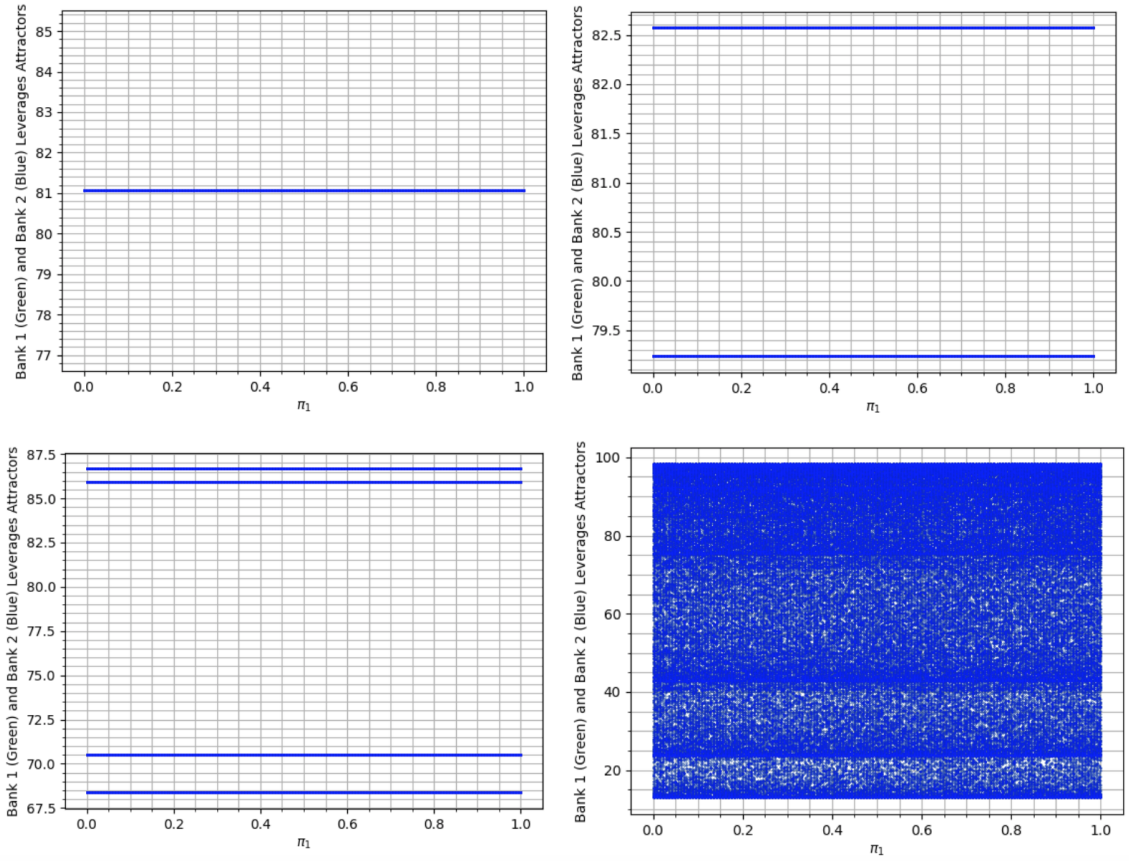

Figure 3: Examples of asymptotic orbits for the two banks as  $\pi_1$  varies and for different choices of  $\omega_1, \omega_2$ . From top to bottom, left to right, it is  $\omega_1 = \omega_2 = 0.8, 0.6, 0.5, 0.3$ . In doing the plots, the first 1000 values have been discarded and the next 500 plotted.

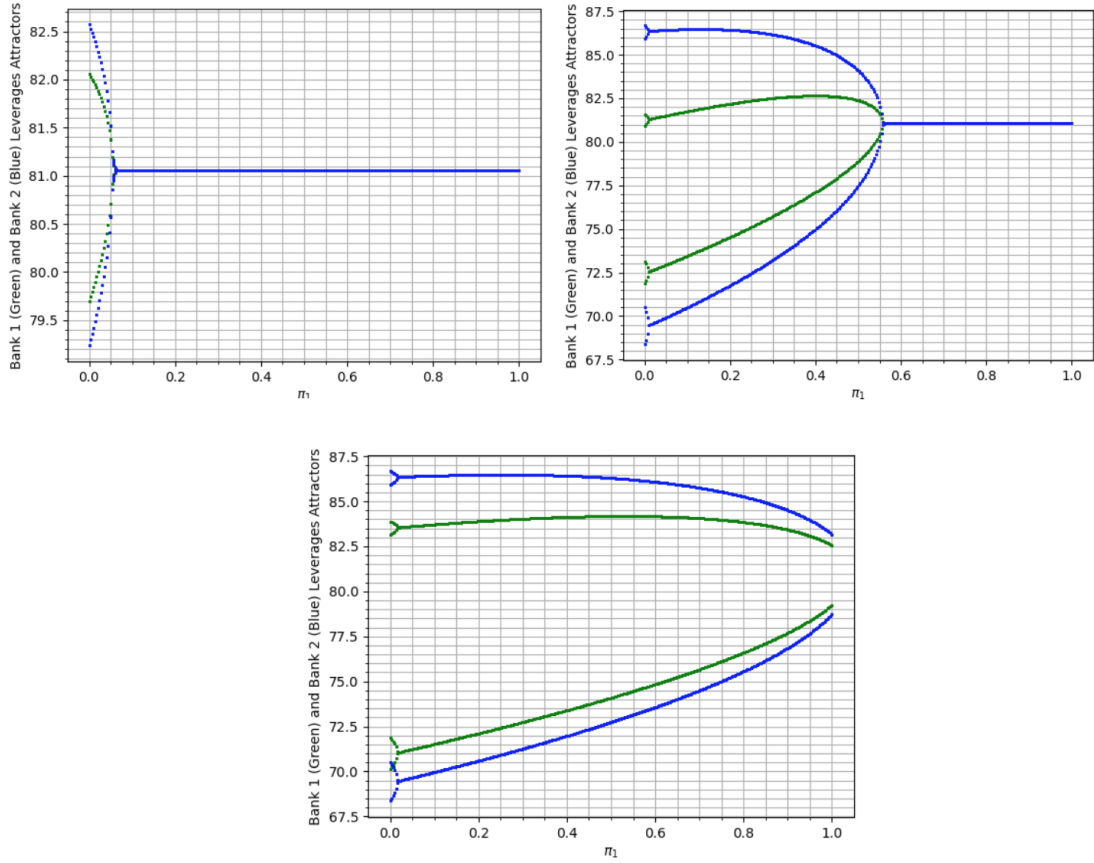

Figure 4: Examples of asymptotic orbits for the two banks as  $\pi_1$  varies and for different choices of  $\omega_1, \omega_2$ . In particular, from top to bottom, left to right, it is:  $\omega_1 = 0.8, \omega_2 = 0.6$ ,  $\omega_1 = 0.8, \omega_2 = 0.5$ , and  $\omega_1 = 0.6, \omega_2 = 0.5$ . In doing the plots, the first 1000 values have been discarded and the next 500 plotted.

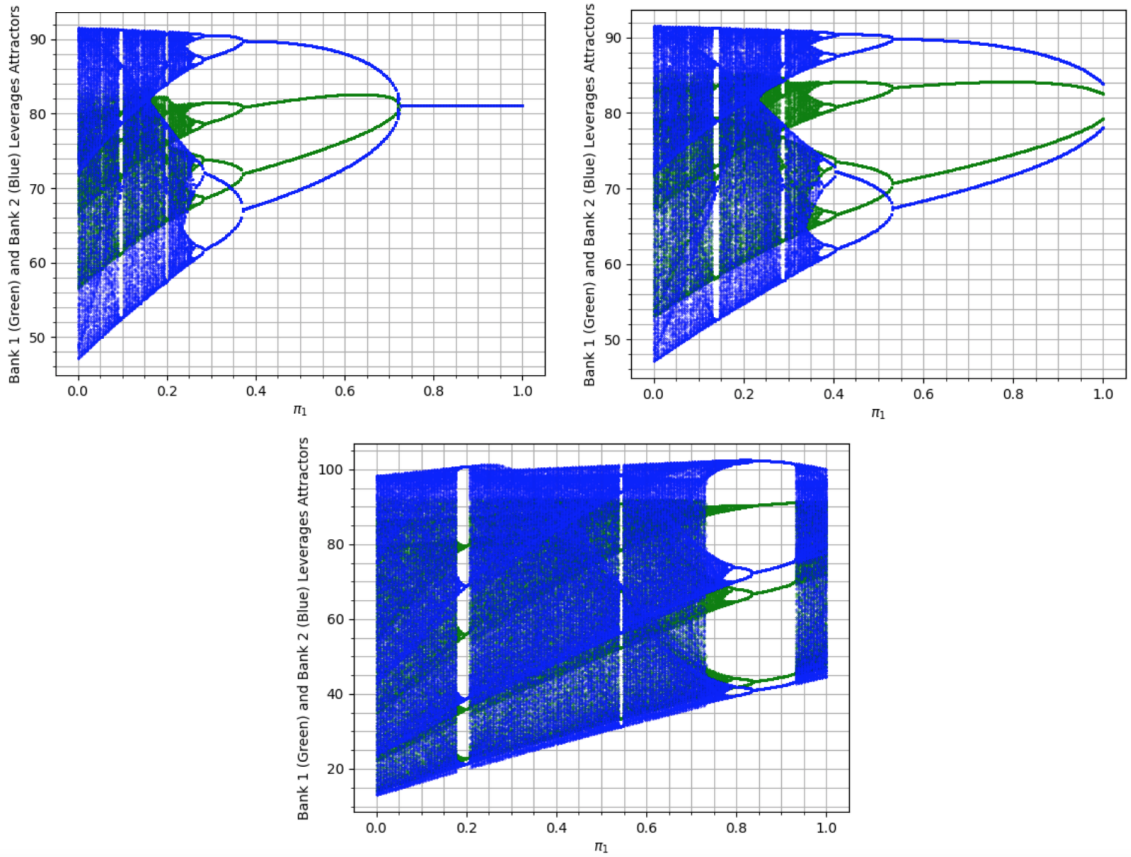

Figure 5: Examples of asymptotic orbits for the two banks as  $\pi_1$  varies and for different choices of  $\omega_1, \omega_2$ . In particular, from top to bottom, left to right, it is:  $\omega_1 = 0.8, \omega_2 = 0.3$ ,  $\omega_1 = 0.6, \omega_2 = 0.3$ , and  $\omega_1 = 0.4, \omega_2 = 0.3$ . In doing the plots, the first 1000 values have been discarded and the next 500 plotted.

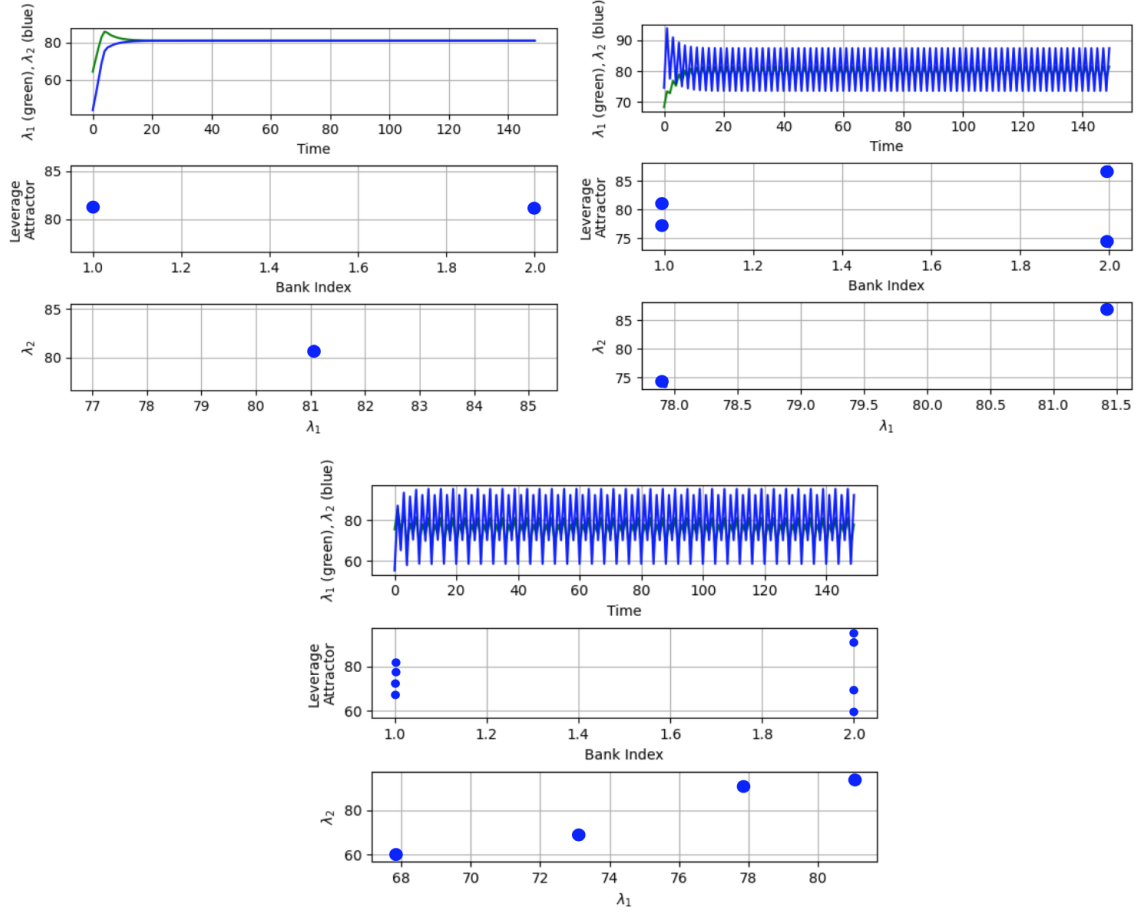

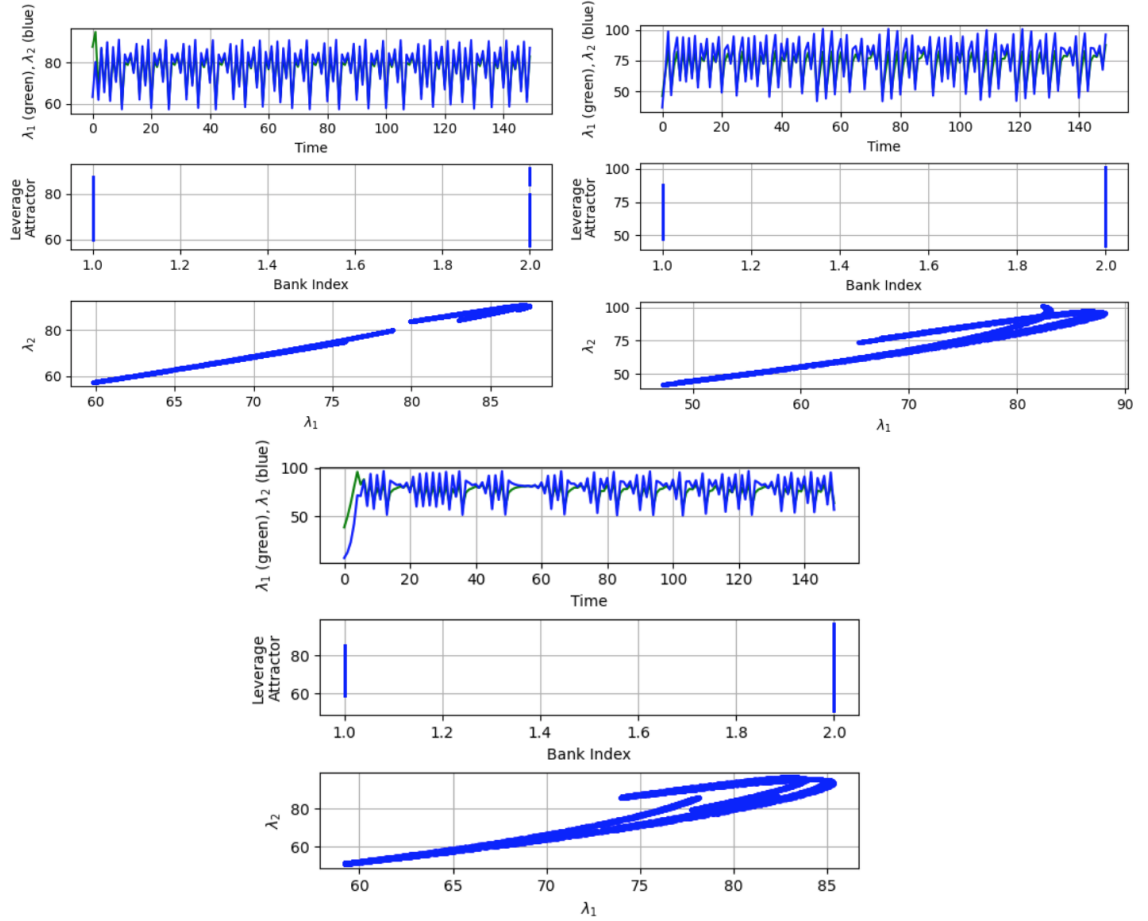

Figure 7: Examples of evolution vs time (top panels), asymptotic orbits for each bank (middle panels) and asymptotic orbits on the  $\lambda_1$  vs  $\lambda_2$  plane (bottom panels) for the two banks for different choices of  $\omega_1, \omega_2, \pi_1$ . In particular, from top to bottom, left to right, it is:  $\omega_1 = 0.5, \omega_2 = 0.4, \pi_1 = 0.5$ ,  $\omega_1 = 0.5, \omega_2 = 0.3, \pi_1 = 0.5$ , and  $\omega_1 = 0.6, \omega_2 = 0.3, \pi_1 = 0.5$ . In doing the plots, the first 1000 values have been discarded and the next 500 plotted.

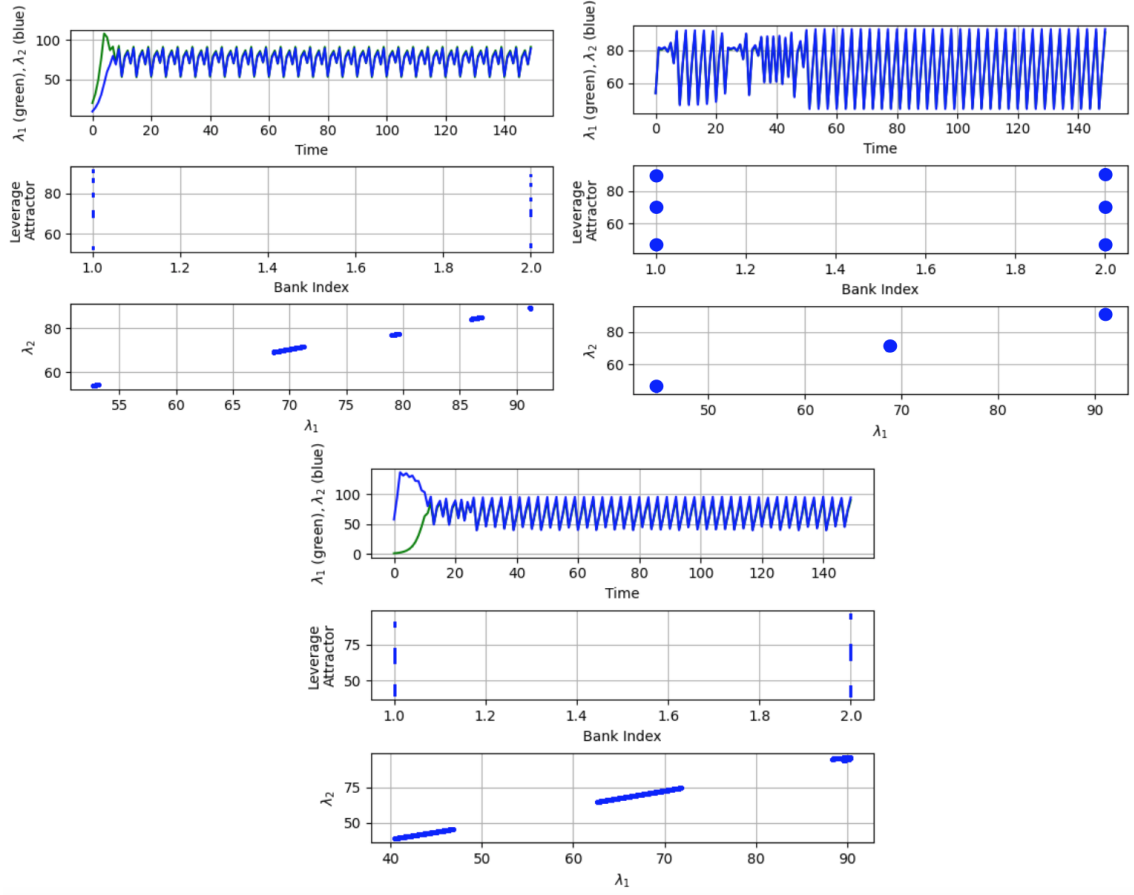

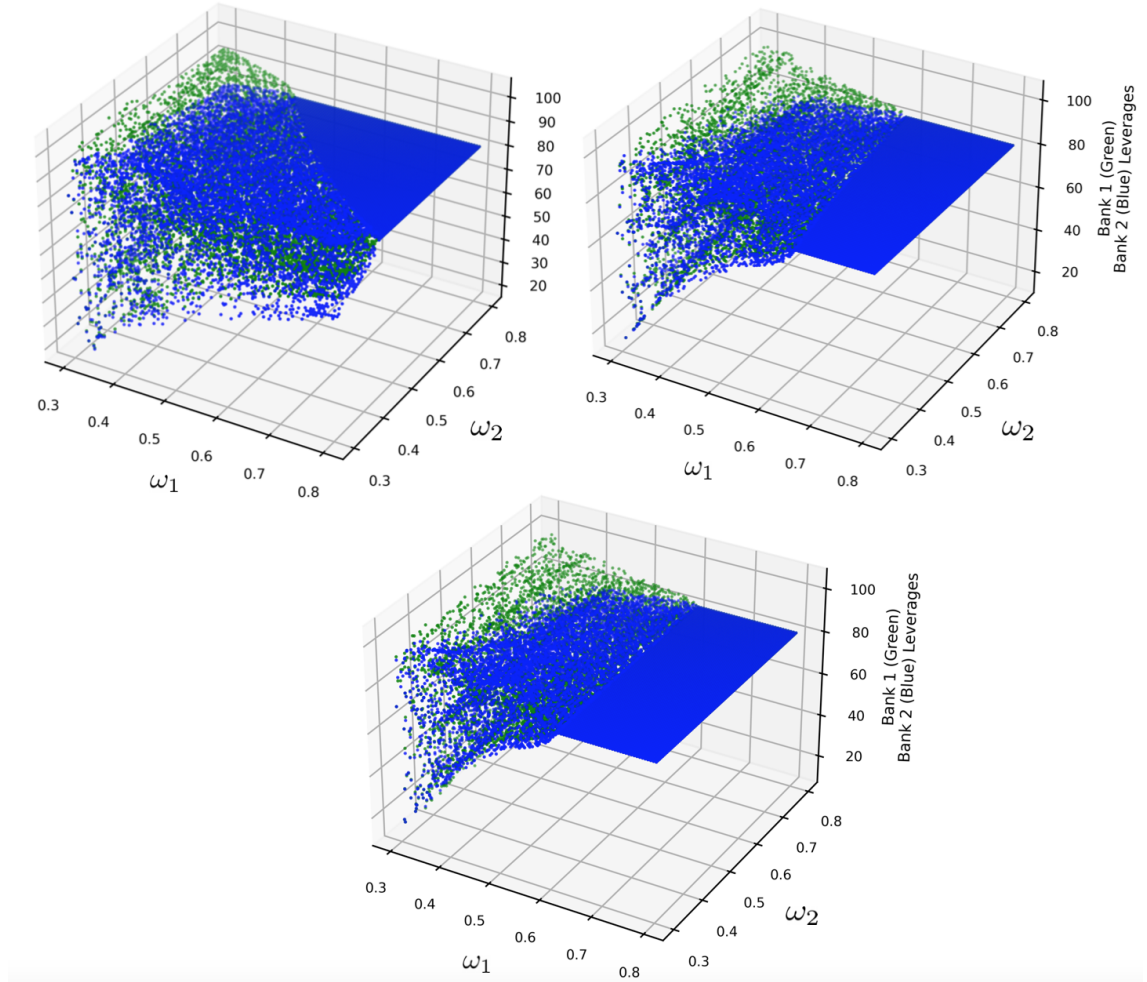

Figure 9: Examples of asymptotic orbits for the two banks as  $\omega_1, \omega_2$  vary for a given choice of  $\pi_1$ . In particular, from top to bottom, left to right, it is:  $\pi_1 = 0.5, 0.9, 0.99$ . In doing the plots, the first 300 values have been discarded and the next 50 plotted.

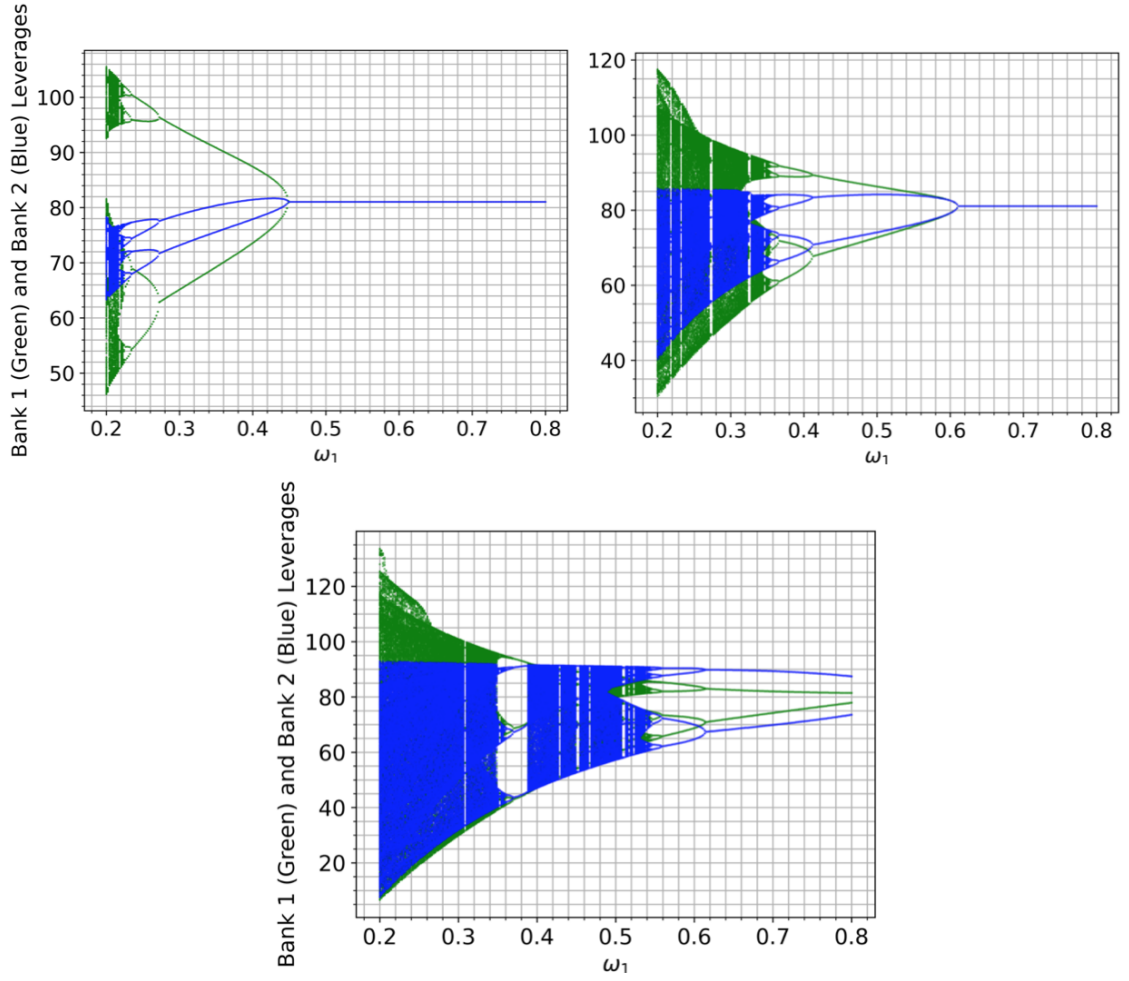

Figure 10: Examples of asymptotic orbits for the two banks as  $\omega_1$  varies for given choices of  $\pi_1 = 0.5$  and  $\omega_2 = 0.8, 0.6, 0.4$  (from top to bottom, left to right). In doing the plots, the first 1000 values have been discarded and the next 800 plotted.

Before proceeding, recall that the leverage of bank 2 satisfies:

$$\lambda_{2,t+1} = T(\lambda_{2,t})$$

with

$$T(x) = \left( \frac{\omega_2}{x^2} + \frac{(1 - \omega_2)\gamma^2\alpha^2\Sigma_\epsilon}{(1 + \gamma - x)^2} \right)^{-\frac{1}{2}}$$

the unimodal map on the interval  $[0, 1 + \gamma]$  with  $T(0) = T(1 + \gamma) = 0$  already introduced. By definition of the leverage it is required that, for every  $t \in \mathbb{N}$ ,  $\lambda_{2,t} \geq 1$ , while stationarity condition of the AR(1) process of the (single) asset in which the two banks are assumed to invest requires  $\frac{\lambda_{2,t}-1}{\gamma} \leq 1$ . For reasonable choices of parameters (comprising the choices made in simulations, e.g.  $\alpha = 1.64$ ,  $\Sigma_\epsilon = 0.0015^2$ ,  $\gamma = 100$ ), the two conditions  $\lambda_{2,t} \geq 1$ ,  $\frac{\lambda_{2,t}-1}{\gamma} \leq 1$  are always verified provided  $\lambda_{2,0} \in [1, T_M^{-1}(1)] \doteq I$  where  $T_M^{-1}(1)$  is the largest preimage of  $\{1\}$  under  $T$  in  $[0, 1 + \gamma]$ .  $T$  has a non flat critical point given by  $\frac{1+\gamma}{1 + \left(\frac{1-\omega_2}{\omega_2}\Sigma_\epsilon\alpha^2\gamma^2\right)^{\frac{1}{3}}}$  and a non zero fixed point

given by  $\frac{1+\gamma}{1+\alpha\gamma\sqrt{\Sigma_\epsilon}}$ . Further, numerical simulations for all the parameters considered in the simulations show evidence that the map  $T$  has negative Schwarzian derivative on  $I$  (in particular for every  $\omega_2 \in [0, 1]$ ,  $\alpha = 1.64$ ,  $\Sigma_\epsilon = 0.0015$ ,  $\gamma = 100$ , but the continuity of the Schwarzian derivative implies this to hold at least in a neighborhood of these values). As for the leverage of bank 1  $\lambda_{1,t}$ , its dynamics depends on bank 2 as well. In particular, introduce the family of maps  $f_y$ , with  $y \in I$ , such that:

$$\lambda_{1,t+1} = f_{\lambda_{2,t}}(\lambda_{1,t})$$

with

$$f_y(x) = \left( \frac{\omega_1}{x^2} + \frac{(1 - \omega_1)\gamma^2\alpha^2\Sigma_\epsilon}{(1 + \gamma - y)^2} \right)^{-\frac{1}{2}}$$

Concerning the constraints, it is required that  $\lambda_{1,t} \geq 1$ . For suitable parameters (including the one used in the simulations and for which the constraints on  $\lambda_{2,t}$  are satisfied) it holds that  $f_{T_M^{-1}(1)}(1) > 1$ , ensuring that the condition  $\lambda_{1,t} \geq 1$  is also always verified.

Notice that, for every allowed choice of  $y \in I$ , the maps  $f_y$  are concave, monotonically increasing with a horizontal asymptote equal to  $\frac{1+\gamma-y}{\gamma\alpha\sqrt{(1-\omega_1)\Sigma_\epsilon}}$ . See Fig. 11 for a qualitative sketch of one of some of these maps.

Furthermore, all these maps have a non zero fixed point given by  $\phi_{f_y} \doteq \frac{1+\gamma-y}{\gamma\alpha\sqrt{\Sigma_\epsilon}}$ , and the derivative of  $f_y$  in  $\phi_{f_y}$  is equal to  $f_y(\phi_{f_y})^3 \frac{\omega_1}{\phi_{f_y}^3} = \omega_1 \in [0, 1]$ .

It is interesting to note that, putting  $\mu_t = \lambda_{2,t}^2$ , one has,  $\forall t \in \mathbb{N}$

$$\mu_{t+1} = \frac{\mu_t}{\omega_1 + A(\lambda_{2,t})\mu_t}$$

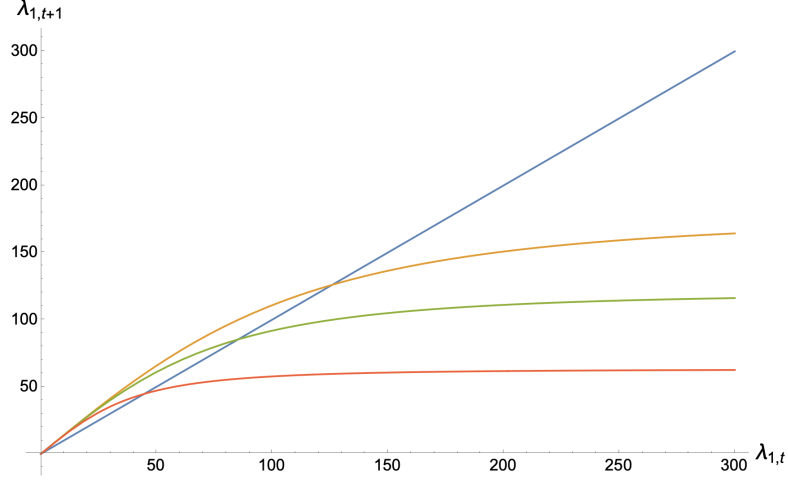

Figure 11: Some maps from the family of maps  $f_y$  with  $y = 70$  (Orange),  $y = 80$  (Green),  $y = 90$  (Red). Here  $\alpha = 1.64$ ,  $\Sigma_\epsilon = 0.0015^2$ ,  $\gamma = 100$ ,  $\omega_1 = 0.5$ . The blue line is the bisector of the first quadrant.

and, for  $n \in \mathbb{N}$ :

$$\mu_{t+n} = \frac{\mu_t}{\omega_1^n + (\sum_{i=0}^{n-1} \omega_1^i A(T^{n-1-i}(\lambda_{2,t})))\mu_t}$$

In particular, the evolution of  $\mu_t$  is described by a Möbius transformation whose parameters change at each iteration and depend on the dynamics of the forcing.

Now some analytical results for this forced-forcing system will be provided.

**Theorem 2.** (*Synchronization on the Fiber*)

$$\forall \lambda \in \hat{I}, \forall (\lambda_{1,0}, \lambda'_{1,0}) \in [1, \infty)^2 : \lim_{n \rightarrow \infty} |\lambda_{1,n} - \lambda'_{1,n}| = 0$$

*That is, the leverages of the forced bank asymptotically synchronize, independently of the initial conditions.*

*Proof.* To prove the statement, call  $a_{\lambda_2} \doteq \frac{1+\gamma-\lambda_2}{\gamma\alpha\sqrt{(1-\omega_1)\Sigma_\epsilon}}$  the asymptote of  $f_{\lambda_2}$ . Notice that,  $\forall \lambda_2 \in I$   $a_{T_M^{-1}(1)} \leq a_{\lambda_2} \leq a_1$ . Moreover, from the previous discussion  $f_{T_M^{-1}(1)}(1) > 1$ , and thus  $a_{T_M^{-1}(1)} > 1$  from the monotonicity of  $f_{T_M^{-1}(1)}$ . Consider the invertible extension of  $T$ ,  $\hat{T} : \hat{I} \rightarrow \hat{I}$  where

$$\hat{I} \doteq \{(\lambda_{2,i})_{i \in \mathbb{Z}} : T(\lambda_{2,i}) = \lambda_{2,i+1} \forall i \in \mathbb{Z}\}$$

such that

$$\hat{T}((\lambda_{2,i})_{i \in \mathbb{Z}}) = (\lambda_{2,i+1})_{i \in \mathbb{Z}}$$

Now put

$$f_{\hat{T}^{-n}(\boldsymbol{\lambda})}^n = f_{\lambda_{2,-1}} \circ \cdots \circ f_{\lambda_{2,-n+1}} \circ f_{\lambda_{2,-n}}$$

where  $\boldsymbol{\lambda} = (\lambda_{2,i})_{i \in \mathbb{Z}} \in \hat{I}$ . Define the function  $x : \hat{I} \rightarrow \mathbb{R}$  by

$$x(\boldsymbol{\lambda}) \doteq \limsup_{n \rightarrow \infty} f_{\hat{T}^{-n}(\boldsymbol{\lambda})}^n(a_{\lambda_{2,-n}})$$

Notice that, from the monotonicity of  $f_{\lambda_{2,-1}}$  one has  $x(\boldsymbol{\lambda}) \leq a_{\lambda_{2,-1}} \forall \boldsymbol{\lambda} \in \hat{I}$ .

Furthermore, since as previously noticed  $f_{\lambda_{2,-1}}(\lambda_1) > f_{\lambda_{2,-1}}(1) > f_{T_M^{-1}(1)}(1) > 1 \forall \lambda_{2,-1} \in I, \forall \lambda_1 \geq 1$ , it follows that  $x(\boldsymbol{\lambda}) > 1 \forall \boldsymbol{\lambda} \in \hat{I}$ .

Next, observe that  $\forall \boldsymbol{\lambda} \in \hat{I}$ ,  $x(\boldsymbol{\lambda})$  is an equivariant point for the dynamics on the fiber of the skew product system, i.e. it follows from the definition of  $x$  and the continuity of the  $f$ s that

$$f_{\lambda_{2,0}}(x(\boldsymbol{\lambda})) = x(\hat{T}(\boldsymbol{\lambda}))$$

Likewise, for  $i \in \mathbb{Z}$ ,

$$f_{\lambda_{2,i}}(x(\hat{T}^i(\boldsymbol{\lambda}))) = x(\hat{T}^{i+1}(\boldsymbol{\lambda})).$$

From now on let's consider a fixed  $\boldsymbol{\lambda} \in \hat{I}$ .

For  $i \in \mathbb{Z}$ , define a rescaled version of  $f_{\lambda_{2,i}}$  as  $\hat{f}_{\lambda_{2,i}} : \mathbb{R}^+ \rightarrow \mathbb{R}^+$  so that, for  $\lambda_{1,0} \geq 1$ ,

$$\hat{f}_{\lambda_{2,i}}(\lambda_{1,0}) \doteq \frac{f_{\lambda_{2,i}}(\lambda_{1,0}x(\hat{T}^i(\boldsymbol{\lambda})))}{x(\hat{T}^{i+1}(\boldsymbol{\lambda}))}$$

Notice that, from the properties of the  $f$ s and from the fixed point property it follows that the  $\hat{f}$ s are concave functions and that  $\hat{f}_{\lambda_{2,i}}(0) = 0$  and  $\hat{f}_{\lambda_{2,i}}(1) = 1$ .

It then follows that,  $\forall i \in \mathbb{Z}, \forall \lambda_{1,0} > 1$ ,  $\hat{f}_{\lambda_{2,i}}(\lambda_{1,0}) < \lambda_{1,0}$  while  $\forall \lambda_{1,0} < 1$ ,  $\hat{f}_{\lambda_{2,i}}(\lambda_{1,0}) > \lambda_{1,0}$ , so that the sequence  $(\hat{f}_{\lambda_{2,i}}^n(\lambda_{1,0}))_{n \in \mathbb{N}}$  is strictly decreasing (increasing) for every  $\lambda_{1,0} > 1$  ( $\lambda_{1,0} < 1$ ) and thus has a limit, which must then be equal to 1 (this can be seen for example for the  $\lambda_{1,0} > 1$  case assuming instead that the limit is greater than one and obtaining a contradiction from the fact that  $f_{\lambda_{2,i}}(\lambda_{1,0}) - \lambda_{1,0}$  is negative bounded away from zero uniformly for  $\lambda_{2,i} \in I$  if  $\lambda_{1,0} > 1$ ).

Next, it can be easily seen by induction on  $n$  that

$$\hat{f}_{\lambda_{2,i}}^n(\lambda_{1,0}) = \frac{f_{\lambda_{2,i}}^n(\lambda_{1,0}x(\hat{T}^i(\boldsymbol{\lambda})))}{x(\hat{T}^{i+n}(\boldsymbol{\lambda}))}. \quad (1)$$

As a consequence  $\forall \lambda_{1,0} \geq 1, \forall \lambda'_{1,0} \geq 1$  one has

$$\lim_{n \rightarrow \infty} |f_{\lambda_{2,i}}^n(\lambda_{1,0}) - f_{\lambda_{2,i}}^n(\lambda'_{1,0})| = \lim_{n \rightarrow \infty} x(\hat{T}^n(\boldsymbol{\lambda})) \left| \hat{f}_{\lambda_{2,i}}^n \left( \frac{\lambda_{1,0}}{x(\boldsymbol{\lambda})} \right) - \hat{f}_{\lambda_{2,i}}^n \left( \frac{\lambda'_{1,0}}{x(\boldsymbol{\lambda})} \right) \right| = 0$$

thus showing that the dependence of the orbit of the first leverage on the initial condition is asymptotically lost.  $\square$

*Remark.* Note that the above proof is completely analytic.

One can then ask how fast this convergence to the fixed point occurs. The following holds.

**Theorem 3.** (*Negative Lyapunov Exponent on the Fiber*)

$$\forall \boldsymbol{\lambda} \in \hat{I}, \forall \lambda_{1,0} \in [1, \infty) : \Lambda_1(\lambda_{1,0}, \lambda_{2,0}) \doteq \lim_{n \rightarrow \infty} \frac{1}{n} \log |(f_{\boldsymbol{\lambda}}^n)'(\lambda_{1,0})| < 0$$

where  $\lambda_{2,0} = (\boldsymbol{\lambda})_0$ .

The above shows that the Lyapunov Exponent for the dynamics on the fiber of the skew product is negative, independently of the initial conditions.

*Proof.* Recall the notation by which  $f_{\boldsymbol{\lambda}}^n = f_{\lambda_{2,n-1}} \circ f_{\lambda_{2,n-2}} \circ \cdots \circ f_{\lambda_{2,1}} \circ f_{\lambda_{2,0}}$ . One has,  $\forall \lambda_{1,0} \geq 1$ ,

$$[(f_{\boldsymbol{\lambda}}^n)'](\lambda_{1,0}) = x(\hat{T}^n(\boldsymbol{\lambda}))[(\hat{f}_{\boldsymbol{\lambda}}^n)']\left(\frac{\lambda_{1,0}}{x(\boldsymbol{\lambda})}\right)$$

Thinking of  $\hat{f}_{\boldsymbol{\lambda}}^0$  as the identity, it is:

$$[(\hat{f}_{\boldsymbol{\lambda}}^n)']\left(\frac{\lambda_{1,0}}{x(\boldsymbol{\lambda})}\right) = \prod_{k=0}^{n-1} \hat{f}'_{\lambda_{2,k}}\left(\hat{f}_{\boldsymbol{\lambda}}^k\left(\frac{\lambda_{1,0}}{x(\boldsymbol{\lambda})}\right)\right)$$

Now  $\forall k \in \mathbb{N}$   $\hat{f}_{\lambda_{2,k}}(1) = 1$  and  $\hat{f}_{\lambda_{2,k}}$  concave imply  $\hat{f}'_{\lambda_{2,k}}(1) < 1$ . Thus by continuity of  $\hat{f}'_{\lambda_{2,k}}$  it follows that  $\forall k \in \mathbb{N}$  there exist a neighborhood of 1 such that  $\hat{f}'_{\lambda_{2,k}} < 1$  there. More precisely, since  $\hat{f}'_{\lambda_{2,k}}(1)$  depends continuously on  $\lambda_{2,k}$ , which varies on the compact set  $I$ , it follows that  $\exists \epsilon > 0$  (independent of  $k$ ) such that  $\forall k \in \mathbb{N}, \forall x \in [1 - \epsilon, 1 + \epsilon], \hat{f}'_{\lambda_{2,k}}(x) < c < 1$  for  $c \in \mathbb{R}^+$ . As from the previous results  $\lim_{k \rightarrow \infty} \hat{f}_{\boldsymbol{\lambda}}^k\left(\frac{\lambda_{1,0}}{x(\boldsymbol{\lambda})}\right) = 1$ , there exist  $K > 0$  such that  $\forall k \geq K$ ,

$$\left|1 - \hat{f}_{\boldsymbol{\lambda}}^k\left(\frac{\lambda_{1,0}}{x(\boldsymbol{\lambda})}\right)\right| < \epsilon$$

Calling then  $B \doteq \prod_{k=0}^{K-1} \hat{f}'_{\lambda_{2,k}}\left(\frac{\lambda_{1,0}}{x(\boldsymbol{\lambda})}\right)$ , one can write, for sufficiently large  $n$  such that  $n > K$ :

$$[(\hat{f}_{\boldsymbol{\lambda}}^n)']\left(\frac{\lambda_{1,0}}{x(\boldsymbol{\lambda})}\right) = B \prod_{k=K}^{n-1} \hat{f}'_{\lambda_{2,k}}\left(\hat{f}_{\boldsymbol{\lambda}}^k\left(\frac{\lambda_{1,0}}{x(\boldsymbol{\lambda})}\right)\right) < Bc^{n-K}$$

This allows to conclude that  $\exists N > 0$  such that  $\forall n \geq N$ ,

$$[(f_{\boldsymbol{\lambda}}^n)'](\lambda_{1,0}) = x(\hat{T}^n(\boldsymbol{\lambda}))[(\hat{f}_{\boldsymbol{\lambda}}^n)']\left(\frac{\lambda_{1,0}}{x(\boldsymbol{\lambda})}\right) < a_{\lambda_{2,-1}} Bc^{n-K} < 1$$

and therefore

$$\Lambda_1(\lambda_{1,0}, \lambda_{2,0}) = \lim_{n \rightarrow \infty} \frac{1}{n} \log |(f_{\lambda}^n)'(\lambda_{1,0})| < 0.$$

□

*Remark.* Note that the above proof is completely analytic.

Before proceeding, it is worth discussing how the forcing bank may behave. In the following paragraph, the dependence of the behavior of the forcing bank on the memory  $\omega_2$  is analyzed. The results here mentioned will be useful in guiding the investigation of the skew product system.

**Classification of behaviors for the forcing bank** It would be interesting to determine the nature of the asymptotic orbit of the first (the forced one) leverage for different kinds of dynamical behavior of the second one (the forcing one). In doing so, we shall suppose all the parameters to be fixed except for  $\omega_2$ , which will then determine the behavior of the forcing bank. More precisely, fix  $\alpha = 1.64$ ,  $\Sigma_{\epsilon} = 0.0015^2$ ,  $\gamma = 100$ . We are considering the family of maps  $\{T_{\omega}\}$  with  $\omega \in [0, 1]$ .

To begin, it is useful to characterize the asymptotic behavior of the forcing leverage.

**Assumption:** From now on we are going to work under the assumption that *the map  $T$  has negative Schwarzian derivative* for all the chosen values of the parameters above. This fact remains unproved, but is corroborated by all our numerical simulations.

Under the assumption above, one can say that for a given  $\omega$ , there is a unique global attractor for  $T$  for almost every initial condition (see for example [3]).

Next, it can be affirmed (see [1]) that for almost every  $\omega \in [0, 1]$  the map  $T$  will either be periodic or chaotic, where we are referring to the following definition.

**Definition 1.** (*Periodic and Chaotic Maps*)

*We say that a map  $T : I \rightarrow I$  is:*

- *Periodic, if  $T$  has a globally attracting periodic orbit;*
- *Chaotic, if  $T$  is topologically transitive on a finite union of intervals contained in  $I$  and it admits a unique absolutely continuous invariant measure with respect to the Lebesgue measure on  $I$  (which will then be supported on a finite union of intervals).*

Let's now better characterize the set of parameters  $\omega$  for which  $T_{\omega}$  is either periodic or chaotic. In the periodic case, we have the following:

**Theorem 4.** (*Abundance of Periodic Maps*)

*The set of  $\omega$  for which  $T_{\omega}$  is periodic is dense in  $[0, 1]$*

*Proof.* First, recall that an interval map  $f : I \rightarrow I$  satisfies Axiom A if  $f$  has finitely many periodic attractors and if  $(f^n)'$  is uniformly exponentially large in  $n$  outside the basins of the periodic attractors.

In particular, notice that if an  $S$ -unimodal map has a stable periodic attractor then it satisfies Axiom A, and vice versa.

Now, by a Theorem from Kozlovski ([6]), if  $f_\lambda$  is a family of real analytic unimodal maps of an interval, depending in a real-analytic fashion on the parameter and such that the family contains at least one Axiom A map and at least two nonconjugated maps, then the Axiom A maps are dense in the set of parameters.

But in our case all the maps from the family  $\{T_\omega\}$  are  $S$ -unimodal maps, and in this family there exists at least a periodic map and at least two nonconjugated maps (which is for example the case if one has a nontrivial bifurcation diagram as the parameter is varied). From these observations we conclude that indeed the set of parameters for which the system has a periodic attractor is dense in the set of parameters.  $\square$

*Remark.* Note that the only numerically-verified hypothesis in the proof above are the fact that the Schwarzian derivative of the maps in the family  $\{T_\omega\}$  is negative (and that the bifurcation diagram of this family over the parameter  $\omega$  is non-trivial).

Before treating the chaotic case, let's introduce the definition:

**Definition 2.** *Misiurewicz map.* An unimodal map  $f$  with critical point  $c$  is called a Misiurewicz map if it has no periodic attractors and if  $c \notin \omega(c)$

We have the following:

**Theorem 5.** *(Abundance of Chaotic Maps)*

$T_\omega$  is chaotic for  $\omega$  in a subset of  $[0, 1]$  of positive measure.

*Proof.* Let's introduce the following hypotheses (we are following [8] here).

H1:  $f_\lambda$  is a one-parameter family of  $C^2$  unimodal maps on an interval  $I$ ;

H2: Without loss of generality, each  $f_\lambda$  has the same nondegenerate critical point  $c$  (this can always be made the case with a linear change of variable);

H3: Each  $f_\lambda$  has a repelling fixed point on the boundary of  $I$

H4: The map  $(x, \lambda) \mapsto \left(f_\lambda(x), \frac{df_\lambda}{dx}(x), \frac{d^2f_\lambda}{dx^2}(x)\right)$  is  $C^1$ ;

H5: There exists a parameter  $\lambda^*$  for which  $f_{\lambda^*}$  is a Misiurewicz map. Suppose that  $f_{\lambda^*}$  maps the critical point to an unstable periodic cycle  $P^*$  in a finite number of steps.

Given H5, for  $\lambda$  sufficiently close to  $\lambda^*$ , one expects (given the general persistence and smooth variation of hyperbolic sets under small perturbations of the map) to find a point  $x(\lambda) \in I$  and an unstable periodic orbit  $P(\lambda)$  such that:

- the map  $\lambda \mapsto x(\lambda)$  is differentiable;
- $x(\lambda^*) = f_{\lambda^*}(c)$ ;
- $P(\lambda)$  depends continuously on  $\lambda$  and  $P(\lambda^*) = P^*$ ;
- $x(\lambda)$  is mapped onto  $P(\lambda)$  in the same number of steps as  $x(\lambda^*)$ . More specifically, it is required that it is mapped on the corresponding point of  $P(\lambda)$

Having defined the map  $x(\lambda)$  it is possible to introduce the last hypothesis:

H6:  $\frac{d}{d\lambda}(x(\lambda) - f_{\lambda}(c))|_{\lambda=\lambda^*} \neq 0$ .

From a theorem by Benedicks and Carlson ([2]), we can conclude that if  $f_{\lambda}$  satisfies H1 – H6, there exist constants  $\gamma > 0$  and  $C > 0$  and a positive measure set  $E$  of parameters with  $\lambda^*$  as a Lebesgue density point, such that

$$|(f_{\lambda}^n)'(f_{\lambda}(c))| \geq Ce^{\gamma n}$$

for every  $\lambda \in E$  and every  $n \geq 1$ .

We aim now to check the hypothesis of this theorem for our family of maps  $\{T_{\omega}\}$ . Let  $\phi(\omega) = \frac{\gamma+1}{1+\alpha\gamma\sqrt{\Sigma_{\epsilon}}}$  be the non zero fixed point of  $T_{\omega}$ , and recall that the critical point of  $T_{\omega}$  is given by  $c(\omega) = \frac{1+\gamma}{1+(\frac{1-\omega}{\omega}\alpha^2\gamma^2\Sigma_{\epsilon})^{\frac{1}{3}}}$ .

Before proceeding, perform the smooth change of coordinates  $x \mapsto \frac{x}{c(\omega)}$  and accordingly define the family of maps  $\tilde{T}_{\omega}$  so that, in the new coordinates,  $x_{t+1} = \tilde{T}_{\omega}(x_t)$ . Explicitly, one has  $\tilde{T}_{\omega}(x) = \frac{T_{\omega}(xc(\omega))}{c(\omega)}$ . This ensures that the nonzero critical point of each of  $\tilde{T}_{\omega}$  does not depend on  $\omega$ , and more precisely it equals 1. Further, call  $\tilde{\phi}(\omega) = \frac{\phi(\omega)}{c(\omega)}$  the non zero fixed point of  $\tilde{T}_{\omega}$ . We shall prove the claim for  $\tilde{T}_{\omega}$ , from which the thesis follows.

- H1, H2, H3, H4: these are easily verified from the nature of  $\tilde{T}_{\omega}$  and from the regularity properties of the mapping

$$(x, \omega) \mapsto \left( \tilde{T}_{\omega}(x), \frac{d\tilde{T}_{\omega}(x)}{dx}, \frac{d^2\tilde{T}_{\omega}(x)}{dx^2} \right)$$

- H5: to prove the existence of a parameter  $\omega^* \in [0, 1]$  for which  $\tilde{T}_{\omega^*}$  is a Misiurewicz map, one could recall results ensuring that there are indeed uncountable many such  $\omega^*$ . This may be proven by showing that the family  $\tilde{T}_{\omega}$  is a *full* family and using results from kneading theory [4]. However, one can also proceed numerically to explicitly find such an  $\omega^*$ , as we shall do below, following the strategy in [8].

One can numerically check that  $\tilde{T}_{0.44}^3(1) - \tilde{\phi}(0.44) < 0$  and  $\tilde{T}_{0.45}^3(1) - \tilde{\phi}(0.45) < 0$ , so that there is an  $\omega^* \in [0.44, 0.45]$  such that the critical point 1 is mapped, in three steps, into the fixed point. It can be easily checked that the fixed point of  $\tilde{T}_\omega$  is unstable for  $\omega \in [0.44, 0.45]$ . As a result, the critical orbit does not accumulate on the critical point and there are no stable periodic cycles (since, as it can be numerically checked, the  $\tilde{T}_\omega$ s have negative Schwarzian derivative, and thus (see [7]) periodic cycles would attract the orbit of the critical point). Therefore  $\tilde{T}_{\omega^*}$  is a Misiurewicz map.

- H6: we shall verify this hypothesis numerically, considering the  $\omega^*$  value from the previous point. Define the function  $\tilde{\mathcal{T}}(x, \omega) \doteq \tilde{T}_\omega(x)$  (and, for  $n > 1$ ,  $\tilde{\mathcal{T}}^n \doteq \tilde{\mathcal{T}}(\tilde{\mathcal{T}}^{n-1}(x, \omega), \omega)$ ) For  $\omega$  close to  $\omega^*$  define  $\zeta(\omega)$  by

$$\begin{cases} \zeta(\omega^*) = \tilde{\mathcal{T}}(1, \omega^*) \\ \tilde{\mathcal{T}}^2(\zeta(\omega), \omega) = \tilde{\phi}(\omega) \end{cases}$$

Then,  $\zeta(\omega)$  will be close to  $\tilde{\mathcal{T}}(1, \omega)$  with the same type of forward orbit as  $\tilde{\mathcal{T}}(1, \omega^*)$ . Then, put  $\zeta_1(\omega) \doteq \tilde{\mathcal{T}}(\zeta(\omega), \omega)$ . We have:

$$\begin{aligned} \frac{d\tilde{\phi}(\omega)}{d\omega} &= \frac{d}{d\omega} \tilde{\mathcal{T}}(\tilde{\mathcal{T}}(\zeta(\omega), \omega), \omega) = \frac{\partial \tilde{\mathcal{T}}}{\partial x}(\zeta_1(\omega), \omega) \frac{d}{d\omega} \tilde{\mathcal{T}}(\zeta(\omega), \omega) + \frac{\partial \tilde{\mathcal{T}}}{\partial \omega}(\zeta_1(\omega), \omega) \\ &= \frac{\partial \tilde{\mathcal{T}}}{\partial x}(\zeta_1(\omega), \omega) \left( \frac{\partial \tilde{\mathcal{T}}}{\partial x}(\zeta(\omega), \omega) \frac{d\zeta(\omega)}{d\omega} + \frac{\partial \tilde{\mathcal{T}}}{\partial \omega}(\zeta(\omega), \omega) \right) + \frac{\partial \tilde{\mathcal{T}}}{\partial \omega}(\zeta_1(\omega), \omega) \end{aligned}$$

From which:

$$\frac{d\zeta(\omega)}{d\omega} = \frac{\frac{\frac{d\tilde{\phi}(\omega)}{d\omega} - \frac{\partial \tilde{\mathcal{T}}}{\partial \omega}(\zeta_1(\omega), \omega)}{\frac{\partial \tilde{\mathcal{T}}}{\partial x}(\zeta_1(\omega), \omega)} - \frac{\partial \tilde{\mathcal{T}}}{\partial \omega}(\zeta(\omega), \omega)}{\frac{\partial \tilde{\mathcal{T}}}{\partial x}(\zeta(\omega), \omega)}$$

Recalling that  $\zeta(\omega^*) = \tilde{T}_{\omega^*}(1)$  and  $\zeta_1(\omega^*) = \tilde{T}_{\omega^*}^2(1)$ , it can now be numerically checked that

$$\frac{d}{d\omega}(\zeta(\omega) - \tilde{\mathcal{T}}(1, \omega))|_{\omega=\omega^*} \neq 0$$

So we can conclude that there exists an  $\omega^* \in [0.44, 0.45]$  which is a Lebesgue density point for the set of  $\omega$  for which  $\tilde{T}_\omega$ , and thus  $T_\omega$ , has chaotic behavior, and hence the latter is a positive measure Lebesgue set.  $\square$

*Remark.* Note that the only numerically-verified facts in the proof are the hypothesis H5 and H6 above.

From these observations, it is natural to restrict our attention to the case in which the behavior of the forcing bank is either periodic or chaotic, as with probability one the behavior will be of one of these two types (as already observed, see [1]) and none of them is “rare”. Let’s begin with the periodic case.

**Theorem 6.** (*Periodic Forcing*)

*If the dynamics of the forcing bank is periodic, then the dynamics of the forced one will be periodic too (of the same period).*

*Proof.* Let’s start by considering the case in which the second leverage has a fixed point attractor  $\phi_T$  (which will then be equal to  $\phi_T \doteq \frac{\gamma+1}{\alpha\gamma\sqrt{\Sigma_\epsilon}+1}$ ).

Then we claim that  $\forall \lambda_{1,0} \in [1, \infty), \forall \lambda_{2,0} \in I$ , the sequence  $\{(f_{\lambda}^n(\lambda_{1,0}), T^n(\lambda_{2,0}))\}$  will approach  $(\phi_T, \phi_T)$  as  $n \rightarrow \infty$  (where  $\lambda = (\lambda_{2,i})_{i \in \mathbb{Z}} \in \hat{I}$ ).

Let’s now prove this claim. Note that the case  $\omega_2 = 1$  is trivial since in this case  $T_2 = T$  is the identity; in this case, there is no fixed point attractor, but every point is a fixed point and thus, for any  $\lambda_2 \in I$ ,  $\lambda_1$  will approach the non zero fixed point of  $f_{\lambda_{2,0}}$ . Thus it will be assumed  $\omega_2 < 1$  in the following.

Choose  $\lambda_{1,0} \in [1, \infty), \lambda_{2,0} \in I$ . Notice that  $f_{\phi_T}$  has an attracting fixed point in  $\frac{\gamma+1-\phi_T}{\gamma\alpha\sqrt{\Sigma_\epsilon}} = \phi_T$ . Actually, given  $\epsilon > 0$ , there exists  $N_0$  such that for every  $n \geq N_0$ , for every  $x \in [1, \infty)$ ,

$$|f_{\phi_T}^n(x) - \phi| \leq \frac{\epsilon}{2}$$

Next, notice that as  $n \rightarrow \infty$  (and thus  $T^n(\lambda_{2,0}) \rightarrow \phi_T$ ),  $f_{\lambda_{2,n}}$  goes uniformly to  $f_{\phi_T}$ , as follows after noticing that, for every  $n$ ,  $f_{\lambda_{2,n}}(0) = 0$ ,  $f_{\lambda_{2,n}}$  is monotonically increasing on the positive real axis and that the limit  $\lim_{x \rightarrow \infty} f_{\lambda_{2,n}}(x) \in \mathbb{R}$  depends continuously on  $\lambda_{2,n}$ . Given now  $\epsilon > 0$  and calling  $K$  the Lipschitz constant of  $f_{\phi_T}$  on  $[1, \infty)$ , one can find  $N_1 \in \mathbb{N}$  such that for every  $n \geq N_1$ ,

$$\|f_{\lambda}^n - f_{\phi_T}\|_{\infty} < \frac{\epsilon}{2 \sum_{j=0}^{N_0-1} K^j}$$

Putting the pieces together, given  $\epsilon > 0$ , for every  $n \geq N_0 + N_1 - 1$  one has, using the triangle inequality  $N_0$  times:

$$\begin{aligned} |f_{\lambda}^n(\lambda_{1,0}) - \phi_T| &\leq \|f_{\lambda}^n - f_{\phi_T}\|_{\infty} + |f_{\phi_T}(f_{\lambda}^{n-1}(\lambda_{1,0}) - \phi_T)| \\ &\leq \|f_{\lambda}^n - f_{\phi_T}\|_{\infty} + K \|f_{\lambda}^{n-1} - f_{\phi_T}\|_{\infty} + |f_{\phi_T}^2(f_{\lambda}^{n-2}(\lambda_{1,0})) - \phi_T| \\ &\leq \frac{\epsilon}{2 \sum_{j=0}^{N_0-1} K^j} \sum_{j=0}^{N_0-1} K^j + \frac{\epsilon}{2} \leq \epsilon \end{aligned}$$

From which the thesis follows in case of period one. In the more general case in which the second leverage reaches an attractor which is a periodic orbit (of period greater than one), then both leverages will approach two (possibly different, if  $\omega_1 \neq \omega_2$ ) periodic attractors of the same period for every initial condition  $\lambda_{1,0}$  and  $\lambda_{2,0}$ .

This follows from the above proof of the fixed point case by noticing that, if for example the period is two, the sequence  $\lambda_{2,0}, T^2(\lambda_{2,0}), T^4(\lambda_{2,0}), \dots$  will converge to one point of the periodic orbit, while  $T(\lambda_{2,0}), T^3(\lambda_{2,0}), T^5(\lambda_{2,0}), \dots$  will converge to the other one. Considering then that all relevant properties of the functions  $\{f_{\lambda_{2,n}}, n \geq 0\}$  exploited in the proof for the fixed point case still hold for the composition of two of these maps (i.e. they all have a repelling zero fixed point and an attracting non zero fixed point, they are monotonically increasing, they approach a limit as the argument goes to infinity which depends continuously and monotonically on  $\lambda_{2,n}$ ) it is immediate to prove that the sequences

$$\lambda_{1,0}, f_{\lambda_{2,1}} \circ f_{\lambda_{2,0}}(\lambda_{1,0}), f_{\lambda_{2,3}} \circ f_{\lambda_{2,2}} \circ f_{\lambda_{2,1}} \circ f_{\lambda_{2,0}}(\lambda_{1,0}) \dots$$

and

$$f_{\lambda_{2,1}}(\lambda_{1,0}), f_{\lambda_{2,2}} \circ f_{\lambda_{2,1}}(\lambda_{1,0}), f_{\lambda_{2,4}} \circ f_{\lambda_{2,3}} \circ f_{\lambda_{2,2}} \circ f_{\lambda_{2,1}}(\lambda_{1,0}) \dots$$

will both converge. □

*Remark.* Note that the above proof is completely analytic.

Let's now turn to the chaotic case.

**Theorem 7.** (*Chaotic Forcing*)

*If the dynamics of the forcing bank is chaotic, then the dynamics of the forced one is topologically transitive on an open subset of  $[1, \infty)$  (to be specified below).*

*Proof.* As usual, assume the second bank is the forcing one. Let's consider the orbit of  $\lambda_{1,0} = 1$  (for, as before, a fixed  $\lambda \in \hat{I}$  with  $\lambda = (\lambda_{2,i})_{i \in \mathbb{Z}}$ ). Notice that, as there is synchronization of the trajectories of the forced bank, the conclusions will then hold for any of its initial conditions. To simplify the notation define  $A(\lambda_2) \doteq \frac{\gamma^2 \alpha^2 \Sigma_\epsilon}{(1 + \gamma - \lambda_2)^2}$ .

One has, for example:

$$\begin{aligned} f_{\lambda_{2,0}}(1) &= (\omega_1 + A(\lambda_{2,0}))^{-\frac{1}{2}} \\ f_{\lambda_{2,1}} \circ f_{\lambda_{2,0}}(1) &= (\omega_1^2 + \omega_1 A(\lambda_{2,0}) + A(\lambda_{2,1}))^{-\frac{1}{2}} \\ f_{\lambda_{2,1}} \circ f_{\lambda_{2,2}} \circ f_{\lambda_{2,1}}(1) &= (\omega_1^3 + \omega_1^2 A(\lambda_{2,0}) + \omega_1 A(\lambda_{2,1}) + A(\lambda_{2,2}))^{-\frac{1}{2}} \\ &\dots \end{aligned}$$

Put then

$$P_n(\lambda_{2,0})^{-2} = \omega_1^n + \sum_{i=0}^{n-1} A(\lambda_{2,n-1-i}) \omega_1^i = \omega_1^n + \sum_{i=0}^{n-1} A(T(\lambda_{2,0})^{n-1-i}) \omega_1^i$$

So that  $f_\lambda^n(1) = P_n(\lambda_{2,0})$ .

As we are assuming  $T$  to be chaotic (i.e. topologically transitive and with an invariant measure absolutely continuous with respect to Lebesgue), its attractor will consist of a finite union of intervals and will be well defined for almost every initial condition. Call this attractor  $\mathcal{A}_0$  and put  $\mathcal{A} \doteq \mathcal{A}_0 \cap I$ . Let's now proceed with the proof, which will be carried on in two steps: in the first one we define the open subset of the space where  $\lambda_1$  lives and on which we shall focus on to prove transitivity in the second step.

### Step 1

To begin with, we shall show that  $\limsup_{n \rightarrow \infty} P_n(\mathcal{A})$  contains an open interval. This will be done exploiting the chaoticity of  $T$ .

Indeed, chaoticity of the map  $T$  allows to conclude (from a result by Keller [5]) that the Lyapunov exponent associated with it is positive for almost every initial condition.

Furthermore, topological transitivity implies that for a generic (in the topological sense)  $\lambda_{2,0} \in \mathcal{A}$  (which is nonempty as  $I$  is invariant), one has that  $(\lambda_{2,i})_{i \in \mathbb{Z}}$  is dense in  $\mathcal{A}$ . In the following let's consider one such  $\lambda_{2,0}$ . Since each  $P_n$  is continuous,  $(P_n(\lambda_{2,i}))_{i \in \mathbb{Z}}$  is then dense in  $P_n(\mathcal{A})$  for every  $n \in \mathbb{N}$ .

For  $n \in \mathbb{N}$ , consider the derivative

$$P'_n(\lambda_{2,0}) = -\frac{1}{2}P_n^3(\lambda_{2,0}) \left[ \omega_1^{n-1} A'(\lambda_{2,0}) + \sum_{i=0}^{n-2} \omega_1^i A'(T(\lambda_{2,0})^{n-1-i}) \prod_{j=0}^{n-2-i} T'(T^j(\lambda_{2,0})) \right]$$

Now,  $\forall n \in \mathbb{N}, \forall \lambda_{2,0} \in I$ ,

$$P_n^{-3}(\lambda_{2,0}) \leq \left( \omega_1^n + \frac{1 - \omega_1^n}{1 - \omega_1} A(T_M^{-1}(1)) \right)^{\frac{3}{2}} \leq \left( 1 + \frac{A(T_M^{-1}(1))}{1 - \omega_1} \right)^{\frac{3}{2}}$$

(using the monotonicity of  $A$  on  $I$ ).

Further, since the Lyapunov exponent of  $T$  is positive, for almost every  $\lambda_{2,0} \in I$  there exist  $c > 1$  and  $N_1 > 0$  such that  $\forall n \geq N_1, \prod_{i=0}^{n-1} T'(T^i(\lambda_{2,0})) > c$ . As a consequence, the term in square brackets in the expression for  $P'_n(\lambda_{2,0})$  above satisfies:

$$\begin{aligned} & \omega_1^{n-1} A'(\lambda_{2,0}) + \sum_{i=0}^{n-2} \omega_1^i A'(T(\lambda_{2,0})^{n-1-i}) \prod_{j=0}^{n-2-i} T'(T^j(\lambda_{2,0})) \\ & \geq \omega_1^{n-1} A'(1) + A'(1) \sum_{i=n-N_1}^{n-2} \omega_1^i \prod_{j=0}^{n-2-i} T'(T^j(\lambda_{2,0})) + A'(1) c \frac{1 - \omega_1^{N_1+1}}{1 - \omega_1} \end{aligned}$$

(using that  $A'$  attains its minimum (positive) value on  $I$  at 1). Now the first two addends in the RHS above are such that

$$\left| \omega_1^{n-1} A'(1) + A'(1) \sum_{i=n-N_1}^{n-2} \omega_1^i \prod_{j=0}^{n-2-i} T'(T^j(\lambda_{2,0})) \right| \leq M^{N_1-1} A'(1) \omega_1^{n-N_1} \frac{1 - \omega_1^{N_1-1}}{1 - \omega_1}$$

Where  $M$  is the maximum absolute value of the derivative of  $T$  on  $I$  (which is greater than 1).

This allows us to choose  $N_2 \in \mathbb{N}$  such that  $\forall n \geq N_2$ ,

$$\begin{aligned} & \omega_1^{n-1} A'(1) + A'(1) \sum_{i=n-N_1}^{n-2} \omega_1^i \prod_{j=0}^{n-2-i} T'(T^j(\lambda_{2,0})) + A'(1) c \frac{1 - \omega_1^{N_1+1}}{1 - \omega_1} \\ & \geq \frac{1}{2} A'(1) c \frac{1 - \omega_1^{N_1+1}}{1 - \omega_1} > 0 \end{aligned}$$

Putting all together,  $\forall n \geq N_2$  and for almost every  $\lambda_{2,0}$  in  $I$ ,

$$|P'_n(\lambda_{2,0})| \geq \frac{1}{2} \left| \left( 1 + \frac{A(T_M^{-1}(1))}{1 - \omega_1} \right)^{-\frac{3}{2}} \right| \left| \frac{1}{2} A'(1) c \frac{1 - \omega_1^{N_1+1}}{1 - \omega_1} \right| > 0$$

But since  $P_n$  is continuously differentiable on  $I$  for every  $n$ , it follows that  $\forall \lambda_{2,0} \in I$ ,  $|P'_n| \geq d > 0$  for  $d \in \mathbb{R}$ .

Now consider one of the intervals constituting  $\mathcal{A}$  and call it  $I_{\mathcal{A}}$ . Then,  $\forall n \geq N_2$ ,  $m(P_n(I_{\mathcal{A}})) \geq m(I_{\mathcal{A}})d$  ( $m$  stands for the Lebesgue measure). In particular,  $\limsup_{n \rightarrow \infty} m(P_n(\mathcal{A}))$  is positive, and therefore  $m(\limsup_{n \rightarrow \infty} P_n(\mathcal{A}))$  is positive (as  $m(\limsup_{n \rightarrow \infty} P_n(\mathcal{A})) \geq \limsup_{n \rightarrow \infty} m(P_n(\mathcal{A}))$ ).

Furthermore, by continuity each  $P_n(\mathcal{A})$  is a finite union of interval, and therefore  $\limsup_{n \rightarrow \infty} P_n(\mathcal{A})$  has a countable number of connected components, and thus contains at least an interval, as it was to be shown.

## Step 2

Now, we shall show that the orbit of  $\lambda_{1,0} = 1$  (and therefore of every  $\lambda_{1,0} \geq 1$  since there is synchronization of the orbits, as shown before) is dense in  $\limsup_{n \rightarrow \infty} P_n(\mathcal{A})$  (which for the above reasoning contains an interval).

First, note that  $\limsup_{n \rightarrow \infty} P_n(\mathcal{A})$  lies in  $[1, \infty]$ . Indeed,  $\forall n \in \mathbb{N}, \forall \lambda_{2,0} \in I$ ,  $P_n(\lambda_{2,0}) = f_{\lambda}^n(1)$  (where  $(\lambda)_0 = \lambda_{2,0}$ ) and the  $f$ s are greater than 1 on  $[1, \infty)$ .

Let then  $B \subseteq [1, \infty] \cap \limsup_{n \rightarrow \infty} P_n(\mathcal{A})$  be an open set.

Let  $\epsilon > 0$  be such that  $B$  contains an interval  $J$  of length  $\epsilon$ . Call  $J' \subseteq J$  the interval of length  $\frac{\epsilon}{2}$  with the same midpoint as  $J$ .

Next, from the definition of  $P_n$ , there will exist a  $N_3 > 0$  such that  $\forall n \geq N_3$ ,  $|f_{\lambda}^n(1) - P_{N_3}(\lambda_{2,n})| < \frac{\epsilon}{2}$  (since  $\omega_1 < 1$  and  $A$  is a continuous function on the compact set  $I$  and therefore  $A(\lambda_2)$  is bounded for  $\lambda_2 \in I$ ).

Then if for a certain  $n_0 \geq N_3$  one has  $P_{N_3}(\lambda_{2,n_0}) \in J'$  it follows that  $f_{\lambda}^{n_0}(1) \in J \subseteq B$ .

Since  $J' \subseteq \limsup_{n \rightarrow \infty} P_n(\mathcal{A})$ , it can be chosen a  $N_4 \geq N_3$  such that  $P_{N_4}(\mathcal{A}) \cap J' \neq \emptyset$ . Let then  $s_0 \in P_{N_4}(\mathcal{A}) \cap J'$ .

By chaoticity of  $T$ , a generic  $\lambda_{2,0} \in \mathcal{A}$  has a dense orbit in  $\mathcal{A}$ , and thus by continuity of the  $P$ s,  $\forall \epsilon' > 0$  there exists  $N_5 \in \mathbb{N}$  such that  $P_{N_4}(g^{N_5}(\lambda_{2,0})) \in B_{\epsilon'}(s_0)$ . This implies that by choosing  $\epsilon'$  small enough one can find  $N_5$  such that  $f_{\lambda}^{N_5}(1) \in B$ .

The arbitrariness of the open set  $B$  allows then to conclude that the orbit of  $\lambda_{1,0} = 1$  (and therefore of every  $\lambda_{1,0} \geq 1$  since there is synchronization of the orbits, as shown before) is dense at least in  $\limsup_{n \rightarrow \infty} P_n(\mathcal{A})$  for a generic (topologically) initial condition of the forcing bank  $\lambda_{2,0} \in \mathcal{A}$ .  $\square$

*Remark.* Note that the only numerically-verified fact in the above proof is that the Schwarzian derivative of the maps  $T$  is negative (this hypothesis is needed, for instance, to use the results about the positivity of the Lyapunov exponent of  $T$  in the chaotic case).

Actually, one can be more precise on manner in which the orbit on the fiber depends on the orbit on the base.

**Theorem 8.** (*Expression for the Random Fixed Point on the Fiber*)

*One has the following expression for the Fixed Point on the fiber of the skew product system:*

$$x(\lambda) = \frac{1}{\sqrt{\sum_{i=0}^{\infty} A(\lambda_{2,-1-i})\omega_1^i}}$$

where  $A(\lambda) = \frac{\gamma^2 \alpha^2 \Sigma_{\epsilon}}{(1+\gamma-\lambda)^2}$ .

*In particular,  $x$  depends continuously on the parameters and the past orbit of the forcing bank.*

*Proof.* Recall the relation between  $f_{\lambda}^n$ ,  $\hat{f}_{\lambda}^n$  and the fixed point  $x(\lambda)$  on the fiber of the skew product system introduced earlier (cf. Eq. 1):

$$\hat{f}_{\lambda}^n(\lambda_{1,0}) = \frac{f_{\lambda}^n(\lambda_{1,0}x(\lambda))}{x(\hat{T}^n(\lambda))}$$

Put  $\lambda_{1,0} = 1$  and recall that it has been shown that

$$\forall \lambda_{1,0} \in [1, \infty) \lim_{n \rightarrow \infty} \hat{f}_{\lambda}^n(\lambda_{1,0}) = 1$$

Further, since as shown orbits on the fiber synchronize asymptotically,

$$\lim_{n \rightarrow \infty} f_{\lambda}^n(x(\lambda)) = \lim_{n \rightarrow \infty} f_{\lambda}^n(1) = \lim_{n \rightarrow \infty} P_n(\lambda_{2,0})$$

(the  $P_n$ s being as usual defined as in the proof of Th. 7). Putting all of this together, one has the expression for the fixed point:

$$x(\lambda) = \frac{1}{\sqrt{\sum_{i=0}^{\infty} A(\lambda_{2,-1-i})\omega_1^i}}$$

□

*Remark.* Note that the above proof is completely analytic

Thus, for example, it appears that  $x(\lambda)$  depends continuously on  $\omega_1$ . Moreover, if for example one considers  $\hat{I}$  as a metric space with the metric induced by the sup norm,  $x(\lambda)$  defines a continuous function from  $\hat{I}$  to  $\mathbb{R}$ .

Finally, let's go back to the case in which the forcing is chaotic. We know (see for instance theorem 1.2 in Chapter V of [4]) that if  $T$  doesn't have periodic attractors, then it is ergodic with respect to the Lebesgue measure on  $I$ . By chaoticity,  $T$  has a unique absolutely continuous invariant measure, which will then be supported on the attractor constituted by a finite union of intervals (see [4]). It is possible to make estimates on the frequency of visit of an open set by the orbit on the fiber (e.g. by the sequence  $(f_{\lambda}^i(1))_{i \in \mathbb{N}}$ . Recall that every initial condition will asymptotically approach the same orbit, so the choice of 1 as a starting point is not significant). The following holds:

**Theorem 9.** (*Estimates on the Frequency of Visit*) Suppose  $T$  is chaotic and call  $\mu_T$  its unique invariant absolutely continuous invariant measure. Let the family of functions  $\{P_n\}_{n \in \mathbb{N}}$  be defined as in the proof of Th. 7. Lastly, let  $B \subseteq \limsup_{n \rightarrow \infty} P_n(\mathcal{A}) \subseteq [1, \infty)$  be a nonempty open set (which exists by the proof of Th. 7) and  $J'$  an interval contained in  $B$  as in the proof of Th. 7. Then there exists  $N^* \in \mathbb{N}$  such that

$$\forall N \geq N^* \quad \lim_{n \rightarrow \infty} \frac{1}{n} \sum_{i=0}^n \chi_B(f_{\lambda}^i(1)) \geq \mu_T(\{\lambda_2 \in P_{N^*}^{-1}(J')\})$$

*Proof.* Choosing an interval  $J' \subseteq B$  as in the proof of Th. 7, it holds, for  $N \in \mathbb{N}$  large enough:

$$\lim_{n \rightarrow \infty} \frac{1}{n} \sum_{i=0}^n \chi_B(f_{\lambda}^i(1)) \geq \lim_{n \rightarrow \infty} \frac{1}{n} \sum_{i=0}^n \chi_{J'}(P_N(\lambda_{2,i}))$$

where the  $\chi$ s stand for indicator functions.

In this case, one could make the following estimate (which then depends on the choice of  $J'$  and  $N$ ). By Birkhoff ergodic theorem one has, for  $\mu_T$ -almost every  $\lambda_{2,0} \in \mathcal{A}$ :

$$\begin{aligned}
\lim_{n \rightarrow \infty} \frac{1}{n} \sum_{i=0}^n \chi_B(f_{\lambda}^i(1)) &\geq \lim_{n \rightarrow \infty} \frac{1}{n} \sum_{i=0}^n \chi_{J'}(P_N(\lambda_{2,i})) = \lim_{n \rightarrow \infty} \frac{1}{n} \sum_{i=0}^n \chi_{J'}(P_N(g^i(\lambda_{2,0}))) \\
&= \int_I \chi_{J'}(P_N(\lambda_2)) d\mu_T(\lambda_2) = \mu_T(\{\lambda_2 \in P_N^{-1}(J')\})
\end{aligned}$$

□

*Remark.* Again, the above proof relies on the fact that the Shwarzian derivative of the map  $T$  is negative, which is the only fact which has been proven numerically.

By appropriately varying  $J'$  and  $N$  one may then obtain better estimates.

### 2.3.3 The general $\pi \neq 0, 1$ case

As seen in simulations (cf. for example Figs. 4), for  $\omega_1, \omega_2$  such that an isolated bank with  $\omega_2$  would have a fixed point and an isolated bank with  $\omega = \omega_1$  would have a periodic attractor of period at least 2, as  $\pi_1$  is varied from 1 to 0 one observes a sequence of period doubling bifurcations. Indeed, one has:

**Theorem 10.** (*Bifurcation Diagram as a Function of  $\pi_1$* )

*For some choices of parameters (which is made explicit below), a critical value  $\pi_{1,bif}$  exists such that for  $\pi_1 < \pi_{1,bif}$  the system approaches a 2-period attractor and for  $\pi_1 > \pi_{1,bif}$  it approaches a fixed point.*

*Proof.* Consider the Jacobian matrix  $\mathbf{J}_{(\phi_T, \phi_T)}(\pi_1)$  of the map  $(T_1(\lambda_1, \lambda_2), T_2(\lambda_1, \lambda_2))$  at its fixed point as a function of  $\pi_1$ .

To find the fixed point  $(\phi_1, \phi_2)$ , we require  $T_1(\phi_1, \phi_2) = \phi_1$  and  $T_2(\phi_1, \phi_2) = \phi_2$ , i.e.:  $\frac{1}{\phi_1^2} - \frac{\omega_1}{\phi_1^2} = (1 - \omega_1) \frac{\gamma^2 \alpha^2 \Sigma_\epsilon}{(1 + \gamma - \pi_1 \phi_1 - (1 - \pi_1) \phi_2)^2}$  and  $\frac{1}{\phi_2^2} - \frac{\omega_2}{\phi_2^2} = (1 - \omega_2) \frac{\gamma^2 \alpha^2 \Sigma_\epsilon}{(1 + \gamma - \pi_1 \phi_1 - (1 - \pi_1) \phi_2)^2}$ . From these we get  $\phi_1 = \phi_2$  and therefore  $\phi_1 = \phi_2 = \phi_T$  where  $\phi_T$  is the fixed point for the one-dimensional map we already encountered before. Explicitly, our fixed point is given by  $(\phi_T, \phi_T)$  where  $\phi_T = \frac{1 + \gamma}{1 + \gamma \alpha \sqrt{\Sigma_\epsilon}}$ .

Now, one has:

$$\mathbf{J}_{(\phi_T, \phi_T)}(\pi_1) = \phi_T^3 \begin{pmatrix} \frac{\omega_1}{\phi_T^3} - \frac{(1 - \omega_2) \pi_1 \alpha^2 \gamma^2 \Sigma_\epsilon}{(1 + \gamma - \phi_T)^3} & -\frac{(1 - \pi_1)(1 - \omega_1) \alpha^2 \gamma^2 \Sigma_\epsilon}{(1 + \gamma - \phi_T)^3} \\ -\frac{\pi_1(1 - \omega_2) \alpha^2 \gamma^2 \Sigma_\epsilon}{(1 + \gamma - \phi_T)^3} & \frac{\omega_2}{\phi_T^3} - \frac{(1 - \omega_2)(1 - \pi_1) \alpha^2 \gamma^2 \Sigma_\epsilon}{(1 + \gamma - \phi_T)^3} \end{pmatrix}$$

Its determinant  $J_{(\phi_T, \phi_T)}(\pi_1)$  is then:

$$\begin{aligned}
J_{(\phi_T, \phi_T)}(\pi_1) &= \omega_1 \omega_2 - \frac{\omega_1(1 - \pi_1)(1 - \omega_2)}{\alpha \gamma \sqrt{\Sigma_\epsilon}} - \frac{\omega_2 \pi_1(1 - \omega_1)}{\alpha \gamma \sqrt{\Sigma_\epsilon}} \\
&\quad + \pi_1(1 - \pi_1)(1 - \omega_1)(1 - \omega_2) \alpha \gamma \sqrt{\Sigma_\epsilon} - \frac{\pi_1(1 - \pi_1)(1 - \omega_1)(1 - \omega_2)}{\alpha^2 \gamma^2 \Sigma_\epsilon}.
\end{aligned}$$

In particular (as one would expect) it is a polynomial of degree two. To have a period doubling bifurcation,  $J_{(\phi_T, \phi_T)}(\pi_1)$  has to “cross”  $-1$ .

If the coefficient of  $\pi_1^2$  is greater than zero (as it is for the choice made for the parameters), that is if  $\frac{1}{\gamma^2 \alpha^2 \Sigma_\epsilon} - \alpha \gamma \sqrt{\Sigma_\epsilon} > 0$ , a period-doubling bifurcation will occur if:

$$J_{(\phi_T, \phi_T)}(0) + 1 = 1 + \omega_1 \omega_2 - \frac{\omega_1(1 - \omega_2)}{\alpha \gamma \sqrt{\Sigma_\epsilon}} < 0$$

and

$$J_{(\phi_T, \phi_T)}(1) + 1 = 1 + \omega_1 \omega_2 - \frac{\omega_2(1 - \omega_1)}{\alpha \gamma \sqrt{\Sigma_\epsilon}} > 0$$

One can check that this conditions are indeed satisfied for example for the parameters used to obtain the plots in the top row of Fig. 4.

For completeness, by solving the equation  $J_{(\phi_T, \phi_T)}(\pi_{1, \text{bif}}) = -1$  one obtains an expression for the weight  $\pi_{1, \text{bif}} = \frac{-c_2 + \sqrt{c_2^2 - 4c_1 c_3}}{2c_1}$  at which the bifurcation from period one to period two occurs (if the above conditions hold), where

$$\begin{aligned} c_1 &= -(1 - \omega_1)(1 - \omega_2)\alpha\gamma\sqrt{\Sigma_\epsilon} + \frac{(1 - \omega_1)(1 - \omega_2)}{\alpha^2\gamma^2\Sigma_\epsilon} \\ c_2 &= (1 - \omega_1)(1 - \omega_2)\alpha\gamma\sqrt{\Sigma_\epsilon} + \frac{\omega_1 - \omega_2}{\alpha\gamma\sqrt{\Sigma_\epsilon}} - \frac{(1 - \omega_1)(1 - \omega_2)}{\alpha^2\gamma^2\Sigma_\epsilon} \\ c_3 &= \omega_1\omega_2 - \frac{\omega_1(1 - \omega_2)}{\alpha\gamma\sqrt{\Sigma_\epsilon}} + 1 \end{aligned}$$

□

*Remark.* Note that the above proof is completely analytic.

In some sense,  $\pi_{1, \text{bif}}$  represents a critical value for which the system undergoes a bifurcation, qualitatively changing its asymptotic behavior. If one is instead interested in the bifurcation that leads from period  $2^n$  to period  $2^{n+1}$ , one might apply the reasoning above to the  $n$ -th iteration of the map in order to determine where this bifurcation occurs.

**Fractal attractor** As observed, for a certain choice of parameters, an Hénon-like attractor is observed (cf., for example, Fig. 7). This may after all not be so surprising as in certain limits one can reduce the system to a perturbed unimodal one.

The box counting dimension for an instance of a Hénon-like attractor (in the case in which  $\pi_1 = 0.5, \omega_1 = 0.5, \omega_2 = 0.3$ ) has been calculated with the usual algorithm (considering 10 box length logarithmically spaced between 0.1 and 1 and then performing a least square fit with a line whose slope was taken as the box counting

dimension. The uncertainty on this value has been estimated as the standard deviation of the slopes of the 9 lines through the point corresponding to the largest box and the 9 other points) obtaining  $1.203 \pm 0.006$ .

## References

- [1] Artur Avila, Mikhail Lyubich, and Welington De Melo. “Regular or stochastic dynamics in real analytic families of unimodal maps”. In: *Inventiones mathematicae* 154.3 (2003), pp. 451–550.
- [2] Michael Benedicks and Lennart Carleson. “The dynamics of the Hénon map”. In: *Annals of Mathematics* 133.1 (1991), pp. 73–169.
- [3] Alexander M Blokh and M Yu Lyubich. “Measurable dynamics of  $S$ -unimodal maps of the interval”. In: *Annales scientifiques de l’Ecole normale supérieure*. Vol. 24. 5. 1991, pp. 545–573.
- [4] Welington De Melo and Sebastian Van Strien. *One-dimensional dynamics*. Vol. 25. Springer Science & Business Media, 2012.
- [5] Gerhard Keller. “Exponents, attractors and Hopf decompositions for interval maps”. In: *Ergodic Theory and Dynamical Systems* 10.4 (1990), pp. 717–744.
- [6] OLEG Kozlovski. “Structural stability in 1D dynamics”. In: *This page intentionally left blank* (2003), p. 107.
- [7] David Singer. “Stable orbits and bifurcation of maps of the interval”. In: *SIAM Journal on Applied Mathematics* 35.2 (1978), pp. 260–267.
- [8] Hans Thunberg. “Periodicity versus chaos in one-dimensional dynamics”. In: *SIAM review* 43.1 (2001), pp. 3–30.
